# Supplementary material for: Neutron knockout in neutral-current neutrino-oxygen interactions
Source: arXiv:1305.2068 ancillary file (2013-11-13)
Supplement: Supplementary file 1 [file Tables.pdf]

# Neutron knockout in neutral-current neutrino-oxygen interactions. Supplemental Material

Artur M. Ankowski and Omar Benhar
*INFN and Department of Physics, "Sapienza" Università di Roma, I-00185 Roma, Italy*

In the following tables, we present as a function of energy the calculated cross sections for ${}^{16}_{8}\mathrm{O}(\nu,\nu')$ and ${}^{16}_{8}\mathrm{O}(\bar\nu,\bar\nu')$ scattering (labeled as "total"), as well as those for neutron knockout induced by the interaction (labeled as "neutrons"). The results are reported for three values of the strange axial coupling constant. The energy is expressed in GeV, and the cross sections are given in units of $10^{-38}$ cm$^2$.

TABLE I: The neutrino cross sections.

| $E_\nu$ (GeV) | total ($g_A^s = -0.03$) | neutrons ($g_A^s = -0.03$) | total ($g_A^s = -0.08$) | neutrons ($g_A^s = -0.08$) | total ($g_A^s = -0.13$) | neutrons ($g_A^s = -0.13$) |
|---|---|---|---|---|---|---|
| 0.001 | 0.00000e+000 | 0.00000e+000 | 0.00000e+000 | 0.00000e+000 | 0.00000e+000 | 0.00000e+000 |
| 0.002 | 0.00000e+000 | 0.00000e+000 | 0.00000e+000 | 0.00000e+000 | 0.00000e+000 | 0.00000e+000 |
| 0.003 | 0.00000e+000 | 0.00000e+000 | 0.00000e+000 | 0.00000e+000 | 0.00000e+000 | 0.00000e+000 |
| 0.004 | 0.00000e+000 | 0.00000e+000 | 0.00000e+000 | 0.00000e+000 | 0.00000e+000 | 0.00000e+000 |
| 0.005 | 0.00000e+000 | 0.00000e+000 | 0.00000e+000 | 0.00000e+000 | 0.00000e+000 | 0.00000e+000 |
| 0.006 | 0.00000e+000 | 0.00000e+000 | 0.00000e+000 | 0.00000e+000 | 0.00000e+000 | 0.00000e+000 |
| 0.007 | 0.00000e+000 | 0.00000e+000 | 0.00000e+000 | 0.00000e+000 | 0.00000e+000 | 0.00000e+000 |
| 0.008 | 2.36049e−014 | 0.00000e+000 | 2.54442e−014 | 0.00000e+000 | 2.73526e−014 | 0.00000e+000 |
| 0.009 | 2.02340e−012 | 0.00000e+000 | 2.18093e−012 | 0.00000e+000 | 2.34438e−012 | 0.00000e+000 |
| 0.010 | 2.75283e−011 | 0.00000e+000 | 2.96698e−011 | 0.00000e+000 | 3.18916e−011 | 0.00000e+000 |
| 0.020 | 1.01690e−006 | 1.02254e−007 | 1.08098e−006 | 9.57253e−008 | 1.14794e−006 | 8.94596e−008 |
| 0.030 | 5.10525e−005 | 1.46215e−005 | 5.29161e−005 | 1.36979e−005 | 5.49195e−005 | 1.28112e−005 |
| 0.040 | 4.36890e−004 | 1.67033e−004 | 4.46917e−004 | 1.56597e−004 | 4.58105e−004 | 1.46572e−004 |
| 0.050 | 1.67693e−003 | 7.24214e−004 | 1.70373e−003 | 6.79439e−004 | 1.73486e−003 | 6.36404e−004 |
| 0.060 | 4.28266e−003 | 1.96733e−003 | 4.33451e−003 | 1.84688e−003 | 4.39718e−003 | 1.73104e−003 |
| 0.070 | 8.69629e−003 | 4.14141e−003 | 8.78074e−003 | 3.89008e−003 | 8.88664e−003 | 3.64824e−003 |
| 0.080 | 1.53177e−002 | 7.46690e−003 | 1.54415e−002 | 7.01738e−003 | 1.56023e−002 | 6.58463e−003 |
| 0.090 | 2.45296e−002 | 1.21529e−002 | 2.46991e−002 | 1.14267e−002 | 2.49268e−002 | 1.07273e−002 |
| 0.100 | 3.67083e−002 | 1.84052e−002 | 3.69290e−002 | 1.73131e−002 | 3.72353e−002 | 1.62608e−002 |
| 0.110 | 5.22103e−002 | 2.64208e−002 | 5.24869e−002 | 2.48638e−002 | 5.28830e−002 | 2.33628e−002 |
| 0.120 | 7.13495e−002 | 3.63773e−002 | 7.16860e−002 | 3.42479e−002 | 7.21829e−002 | 3.21942e−002 |
| 0.130 | 9.43756e−002 | 4.84196e−002 | 9.47741e−002 | 4.56039e−002 | 9.53813e−002 | 4.28872e−002 |
| 0.140 | 1.21456e−001 | 6.26509e−002 | 1.21917e−001 | 5.90313e−002 | 1.22644e−001 | 5.55375e−002 |
| 0.150 | 1.52664e−001 | 7.91244e−002 | 1.53188e−001 | 7.45822e−002 | 1.54039e−001 | 7.01964e−002 |
| 0.160 | 1.87972e−001 | 9.78411e−002 | 1.88557e−001 | 9.22597e−002 | 1.89539e−001 | 8.68687e−002 |
| 0.170 | 2.27255e−001 | 1.18749e−001 | 2.27898e−001 | 1.12016e−001 | 2.29014e−001 | 1.05512e−001 |
| 0.180 | 2.70289e−001 | 1.41739e−001 | 2.70984e−001 | 1.33751e−001 | 2.72236e−001 | 1.26032e−001 |
| 0.190 | 3.16745e−001 | 1.66649e−001 | 3.17488e−001 | 1.57313e−001 | 3.18875e−001 | 1.48287e−001 |
| 0.200 | 3.66222e−001 | 1.93272e−001 | 3.67006e−001 | 1.82505e−001 | 3.68526e−001 | 1.72094e−001 |
| 0.210 | 4.18254e−001 | 2.21361e−001 | 4.19072e−001 | 2.09097e−001 | 4.20722e−001 | 1.97235e−001 |
| 0.220 | 4.72341e−001 | 2.50655e−001 | 4.73189e−001 | 2.36841e−001 | 4.74967e−001 | 2.23477e−001 |
| 0.230 | 5.28001e−001 | 2.80888e−001 | 5.28871e−001 | 2.65486e−001 | 5.30769e−001 | 2.50584e−001 |
| 0.240 | 5.84777e−001 | 3.11813e−001 | 5.85665e−001 | 2.94799e−001 | 5.87677e−001 | 2.78333e−001 |
| 0.250 | 6.42281e−001 | 3.43210e−001 | 6.43179e−001 | 3.24570e−001 | 6.45304e−001 | 3.06527e−001 |
| 0.260 | 7.00171e−001 | 3.74895e−001 | 7.01077e−001 | 3.54623e−001 | 7.03310e−001 | 3.34999e−001 |
| 0.270 | 7.58192e−001 | 4.06713e−001 | 7.59102e−001 | 3.84813e−001 | 7.61437e−001 | 3.63610e−001 |
| 0.280 | 8.16121e−001 | 4.38537e−001 | 8.17034e−001 | 4.15017e−001 | 8.19466e−001 | 3.92244e−001 |
| 0.290 | 8.73782e−001 | 4.70263e−001 | 8.74689e−001 | 4.45137e−001 | 8.77216e−001 | 4.20805e−001 |
| 0.300 | 9.31015e−001 | 5.01806e−001 | 9.31916e−001 | 4.75090e−001 | 9.34538e−001 | 4.49216e−001 |
| 0.310 | 9.87709e−001 | 5.33087e−001 | 9.88609e−001 | 5.04802e−001 | 9.91312e−001 | 4.77407e−001 |
| 0.320 | 1.04377e+000 | 5.64051e−001 | 1.04465e+000 | 5.34218e−001 | 1.04744e+000 | 5.05322e−001 |
| 0.330 | 1.09908e+000 | 5.94635e−001 | 1.09996e+000 | 5.63281e−001 | 1.10283e+000 | 5.32909e−001 |
| 0.340 | 1.15358e+000 | 6.24801e−001 | 1.15445e+000 | 5.91953e−001 | 1.15740e+000 | 5.60129e−001 |
| 0.350 | 1.20721e+000 | 6.54506e−001 | 1.20807e+000 | 6.20189e−001 | 1.21109e+000 | 5.86942e−001 |
| 0.360 | 1.25990e+000 | 6.83709e−001 | 1.26075e+000 | 6.47953e−001 | 1.26385e+000 | 6.13311e−001 |
| 0.370 | 1.31160e+000 | 7.12396e−001 | 1.31245e+000 | 6.75234e−001 | 1.31562e+000 | 6.39224e−001 |
| 0.380 | 1.36229e+000 | 7.40526e−001 | 1.36312e+000 | 7.01986e−001 | 1.36637e+000 | 6.64641e−001 |
| 0.390 | 1.41194e+000 | 7.68082e−001 | 1.41275e+000 | 7.28195e−001 | 1.41607e+000 | 6.89545e−001 |
| 0.400 | 1.46048e+000 | 7.95063e−001 | 1.46129e+000 | 7.53862e−001 | 1.46469e+000 | 7.13937e−001 |
| 0.410 | 1.50795e+000 | 8.21446e−001 | 1.50875e+000 | 7.78963e−001 | 1.51221e+000 | 7.37794e−001 |
| 0.420 | 1.55430e+000 | 8.47209e−001 | 1.55509e+000 | 8.03477e−001 | 1.55861e+000 | 7.61095e−001 |
| 0.430 | 1.59952e+000 | 8.72364e−001 | 1.60030e+000 | 8.27416e−001 | 1.60389e+000 | 7.83854e−001 |
| 0.440 | 1.64361e+000 | 8.96895e−001 | 1.64439e+000 | 8.50761e−001 | 1.64804e+000 | 8.06050e−001 |
| 0.450 | 1.68659e+000 | 9.20818e−001 | 1.68736e+000 | 8.73531e−001 | 1.69108e+000 | 8.27702e−001 |
| 0.460 | 1.72842e+000 | 9.44101e−001 | 1.72919e+000 | 8.95695e−001 | 1.73297e+000 | 8.48780e−001 |
| 0.470 | 1.76914e+000 | 9.66780e−001 | 1.76990e+000 | 9.17285e−001 | 1.77375e+000 | 8.69313e−001 |
| 0.480 | 1.80875e+000 | 9.88843e−001 | 1.80951e+000 | 9.38289e−001 | 1.81342e+000 | 8.89292e−001 |
| 0.490 | 1.84725e+000 | 1.01030e+000 | 1.84801e+000 | 9.58718e−001 | 1.85197e+000 | 9.08724e−001 |
| 0.500 | 1.88467e+000 | 1.03115e+000 | 1.88543e+000 | 9.78572e−001 | 1.88945e+000 | 9.27611e−001 |
| 0.510 | 1.92101e+000 | 1.05141e+000 | 1.92177e+000 | 9.97862e−001 | 1.92585e+000 | 9.45963e−001 |
| 0.520 | 1.95630e+000 | 1.07108e+000 | 1.95705e+000 | 1.01659e+000 | 1.96119e+000 | 9.63785e−001 |
| 0.530 | 1.99054e+000 | 1.09017e+000 | 1.99130e+000 | 1.03478e+000 | 1.99550e+000 | 9.81087e−001 |

| | | | | | | |
|---|---|---|---|---|---|---|
| 0.540 | 2.02378e+000 | 1.10871e+000 | 2.02454e+000 | 1.05243e+000 | 2.02879e+000 | 9.97885e−001 |
| 0.550 | 2.05600e+000 | 1.12669e+000 | 2.05676e+000 | 1.06956e+000 | 2.06107e+000 | 1.01418e+000 |
| 0.560 | 2.08726e+000 | 1.14412e+000 | 2.08802e+000 | 1.08616e+000 | 2.09238e+000 | 1.02999e+000 |
| 0.570 | 2.11755e+000 | 1.16102e+000 | 2.11832e+000 | 1.10226e+000 | 2.12273e+000 | 1.04531e+000 |
| 0.580 | 2.14690e+000 | 1.17741e+000 | 2.14768e+000 | 1.11787e+000 | 2.15216e+000 | 1.06017e+000 |
| 0.590 | 2.17535e+000 | 1.19329e+000 | 2.17614e+000 | 1.13300e+000 | 2.18066e+000 | 1.07457e+000 |
| 0.600 | 2.20290e+000 | 1.20867e+000 | 2.20369e+000 | 1.14765e+000 | 2.20827e+000 | 1.08851e+000 |
| 0.610 | 2.22959e+000 | 1.22358e+000 | 2.23040e+000 | 1.16186e+000 | 2.23502e+000 | 1.10203e+000 |
| 0.620 | 2.25543e+000 | 1.23801e+000 | 2.25624e+000 | 1.17561e+000 | 2.26093e+000 | 1.11512e+000 |
| 0.630 | 2.28046e+000 | 1.25199e+000 | 2.28128e+000 | 1.18892e+000 | 2.28601e+000 | 1.12780e+000 |
| 0.640 | 2.30468e+000 | 1.26553e+000 | 2.30551e+000 | 1.20182e+000 | 2.31030e+000 | 1.14008e+000 |
| 0.650 | 2.32813e+000 | 1.27863e+000 | 2.32897e+000 | 1.21430e+000 | 2.33381e+000 | 1.15196e+000 |
| 0.660 | 2.35081e+000 | 1.29131e+000 | 2.35167e+000 | 1.22639e+000 | 2.35656e+000 | 1.16347e+000 |
| 0.670 | 2.37277e+000 | 1.30359e+000 | 2.37364e+000 | 1.23809e+000 | 2.37858e+000 | 1.17461e+000 |
| 0.680 | 2.39402e+000 | 1.31547e+000 | 2.39489e+000 | 1.24941e+000 | 2.39988e+000 | 1.18539e+000 |
| 0.690 | 2.41458e+000 | 1.32698e+000 | 2.41546e+000 | 1.26037e+000 | 2.42050e+000 | 1.19582e+000 |
| 0.700 | 2.43445e+000 | 1.33810e+000 | 2.43536e+000 | 1.27097e+000 | 2.44044e+000 | 1.20591e+000 |
| 0.710 | 2.45369e+000 | 1.34886e+000 | 2.45461e+000 | 1.28122e+000 | 2.45975e+000 | 1.21568e+000 |
| 0.720 | 2.47230e+000 | 1.35928e+000 | 2.47323e+000 | 1.29115e+000 | 2.47841e+000 | 1.22513e+000 |
| 0.730 | 2.49030e+000 | 1.36935e+000 | 2.49124e+000 | 1.30075e+000 | 2.49647e+000 | 1.23427e+000 |
| 0.740 | 2.50770e+000 | 1.37910e+000 | 2.50866e+000 | 1.31004e+000 | 2.51393e+000 | 1.24312e+000 |
| 0.750 | 2.52452e+000 | 1.38853e+000 | 2.52550e+000 | 1.31902e+000 | 2.53082e+000 | 1.25167e+000 |
| 0.760 | 2.54080e+000 | 1.39765e+000 | 2.54179e+000 | 1.32771e+000 | 2.54716e+000 | 1.25995e+000 |
| 0.770 | 2.55654e+000 | 1.40647e+000 | 2.55754e+000 | 1.33612e+000 | 2.56296e+000 | 1.26795e+000 |
| 0.780 | 2.57175e+000 | 1.41501e+000 | 2.57277e+000 | 1.34425e+000 | 2.57823e+000 | 1.27569e+000 |
| 0.790 | 2.58647e+000 | 1.42326e+000 | 2.58751e+000 | 1.35212e+000 | 2.59301e+000 | 1.28318e+000 |
| 0.800 | 2.60069e+000 | 1.43124e+000 | 2.60175e+000 | 1.35972e+000 | 2.60729e+000 | 1.29042e+000 |
| 0.810 | 2.61443e+000 | 1.43896e+000 | 2.61551e+000 | 1.36708e+000 | 2.62111e+000 | 1.29743e+000 |
| 0.820 | 2.62774e+000 | 1.44643e+000 | 2.62883e+000 | 1.37419e+000 | 2.63446e+000 | 1.30420e+000 |
| 0.830 | 2.64059e+000 | 1.45365e+000 | 2.64170e+000 | 1.38107e+000 | 2.64738e+000 | 1.31075e+000 |
| 0.840 | 2.65301e+000 | 1.46063e+000 | 2.65414e+000 | 1.38772e+000 | 2.65986e+000 | 1.31709e+000 |
| 0.850 | 2.66502e+000 | 1.46738e+000 | 2.66617e+000 | 1.39415e+000 | 2.67193e+000 | 1.32321e+000 |
| 0.860 | 2.67664e+000 | 1.47392e+000 | 2.67781e+000 | 1.40038e+000 | 2.68361e+000 | 1.32914e+000 |
| 0.870 | 2.68786e+000 | 1.48023e+000 | 2.68904e+000 | 1.40639e+000 | 2.69489e+000 | 1.33487e+000 |
| 0.880 | 2.69870e+000 | 1.48634e+000 | 2.69991e+000 | 1.41221e+000 | 2.70579e+000 | 1.34040e+000 |
| 0.890 | 2.70919e+000 | 1.49225e+000 | 2.71042e+000 | 1.41784e+000 | 2.71634e+000 | 1.34576e+000 |
| 0.900 | 2.71933e+000 | 1.49796e+000 | 2.72058e+000 | 1.42328e+000 | 2.72654e+000 | 1.35094e+000 |
| 0.910 | 2.72914e+000 | 1.50348e+000 | 2.73039e+000 | 1.42853e+000 | 2.73640e+000 | 1.35595e+000 |
| 0.920 | 2.73860e+000 | 1.50882e+000 | 2.73988e+000 | 1.43362e+000 | 2.74592e+000 | 1.36079e+000 |
| 0.930 | 2.74776e+000 | 1.51399e+000 | 2.74906e+000 | 1.43854e+000 | 2.75514e+000 | 1.36547e+000 |
| 0.940 | 2.75660e+000 | 1.51898e+000 | 2.75792e+000 | 1.44329e+000 | 2.76404e+000 | 1.37000e+000 |
| 0.950 | 2.76516e+000 | 1.52382e+000 | 2.76650e+000 | 1.44790e+000 | 2.77266e+000 | 1.37438e+000 |
| 0.960 | 2.77342e+000 | 1.52848e+000 | 2.77478e+000 | 1.45234e+000 | 2.78098e+000 | 1.37861e+000 |
| 0.970 | 2.78142e+000 | 1.53300e+000 | 2.78279e+000 | 1.45665e+000 | 2.78903e+000 | 1.38271e+000 |
| 0.980 | 2.78912e+000 | 1.53736e+000 | 2.79052e+000 | 1.46080e+000 | 2.79680e+000 | 1.38665e+000 |
| 0.990 | 2.79659e+000 | 1.54159e+000 | 2.79801e+000 | 1.46482e+000 | 2.80433e+000 | 1.39049e+000 |
| 1.000 | 2.80380e+000 | 1.54567e+000 | 2.80524e+000 | 1.46870e+000 | 2.81158e+000 | 1.39418e+000 |
| 1.010 | 2.81077e+000 | 1.54961e+000 | 2.81223e+000 | 1.47246e+000 | 2.81861e+000 | 1.39776e+000 |
| 1.020 | 2.81750e+000 | 1.55343e+000 | 2.81898e+000 | 1.47610e+000 | 2.82541e+000 | 1.40122e+000 |
| 1.030 | 2.82401e+000 | 1.55712e+000 | 2.82551e+000 | 1.47961e+000 | 2.83197e+000 | 1.40456e+000 |
| 1.040 | 2.83029e+000 | 1.56068e+000 | 2.83182e+000 | 1.48300e+000 | 2.83831e+000 | 1.40778e+000 |
| 1.050 | 2.83637e+000 | 1.56414e+000 | 2.83791e+000 | 1.48628e+000 | 2.84444e+000 | 1.41091e+000 |
| 1.060 | 2.84224e+000 | 1.56748e+000 | 2.84380e+000 | 1.48946e+000 | 2.85037e+000 | 1.41393e+000 |
| 1.070 | 2.84792e+000 | 1.57070e+000 | 2.84949e+000 | 1.49253e+000 | 2.85609e+000 | 1.41685e+000 |
| 1.080 | 2.85341e+000 | 1.57382e+000 | 2.85501e+000 | 1.49549e+000 | 2.86163e+000 | 1.41967e+000 |
| 1.090 | 2.85870e+000 | 1.57683e+000 | 2.86032e+000 | 1.49836e+000 | 2.86698e+000 | 1.42240e+000 |
| 1.100 | 2.86381e+000 | 1.57975e+000 | 2.86545e+000 | 1.50113e+000 | 2.87215e+000 | 1.42503e+000 |
| 1.110 | 2.86875e+000 | 1.58256e+000 | 2.87041e+000 | 1.50381e+000 | 2.87714e+000 | 1.42758e+000 |
| 1.120 | 2.87353e+000 | 1.58528e+000 | 2.87521e+000 | 1.50640e+000 | 2.88197e+000 | 1.43004e+000 |
| 1.130 | 2.87814e+000 | 1.58792e+000 | 2.87984e+000 | 1.50890e+000 | 2.88664e+000 | 1.43242e+000 |
| 1.140 | 2.88260e+000 | 1.59046e+000 | 2.88432e+000 | 1.51132e+000 | 2.89115e+000 | 1.43472e+000 |
| 1.150 | 2.88690e+000 | 1.59292e+000 | 2.88863e+000 | 1.51366e+000 | 2.89550e+000 | 1.43694e+000 |
| 1.160 | 2.89106e+000 | 1.59530e+000 | 2.89282e+000 | 1.51592e+000 | 2.89971e+000 | 1.43909e+000 |
| 1.170 | 2.89506e+000 | 1.59760e+000 | 2.89685e+000 | 1.51809e+000 | 2.90378e+000 | 1.44116e+000 |
| 1.180 | 2.89894e+000 | 1.59982e+000 | 2.90074e+000 | 1.52021e+000 | 2.90770e+000 | 1.44316e+000 |
| 1.190 | 2.90268e+000 | 1.60196e+000 | 2.90451e+000 | 1.52224e+000 | 2.91150e+000 | 1.44510e+000 |
| 1.200 | 2.90630e+000 | 1.60404e+000 | 2.90814e+000 | 1.52422e+000 | 2.91516e+000 | 1.44697e+000 |
| 1.210 | 2.90979e+000 | 1.60604e+000 | 2.91165e+000 | 1.52611e+000 | 2.91870e+000 | 1.44877e+000 |
| 1.220 | 2.91315e+000 | 1.60797e+000 | 2.91503e+000 | 1.52795e+000 | 2.92211e+000 | 1.45052e+000 |
| 1.230 | 2.91641e+000 | 1.60984e+000 | 2.91831e+000 | 1.52972e+000 | 2.92542e+000 | 1.45221e+000 |
| 1.240 | 2.91955e+000 | 1.61165e+000 | 2.92147e+000 | 1.53145e+000 | 2.92861e+000 | 1.45384e+000 |
| 1.250 | 2.92257e+000 | 1.61339e+000 | 2.92451e+000 | 1.53310e+000 | 2.93169e+000 | 1.45540e+000 |
| 1.260 | 2.92550e+000 | 1.61508e+000 | 2.92746e+000 | 1.53469e+000 | 2.93466e+000 | 1.45692e+000 |
| 1.270 | 2.92832e+000 | 1.61670e+000 | 2.93029e+000 | 1.53624e+000 | 2.93753e+000 | 1.45838e+000 |
| 1.280 | 2.93104e+000 | 1.61827e+000 | 2.93303e+000 | 1.53773e+000 | 2.94030e+000 | 1.45980e+000 |
| 1.290 | 2.93366e+000 | 1.61979e+000 | 2.93568e+000 | 1.53916e+000 | 2.94297e+000 | 1.46116e+000 |
| 1.300 | 2.93620e+000 | 1.62126e+000 | 2.93823e+000 | 1.54055e+000 | 2.94555e+000 | 1.46248e+000 |
| 1.310 | 2.93864e+000 | 1.62267e+000 | 2.94070e+000 | 1.54189e+000 | 2.94805e+000 | 1.46375e+000 |
| 1.320 | 2.94099e+000 | 1.62403e+000 | 2.94307e+000 | 1.54318e+000 | 2.95044e+000 | 1.46497e+000 |
| 1.330 | 2.94326e+000 | 1.62535e+000 | 2.94535e+000 | 1.54443e+000 | 2.95275e+000 | 1.46616e+000 |
| 1.340 | 2.94545e+000 | 1.62662e+000 | 2.94756e+000 | 1.54563e+000 | 2.95500e+000 | 1.46730e+000 |
| 1.350 | 2.94757e+000 | 1.62784e+000 | 2.94970e+000 | 1.54679e+000 | 2.95715e+000 | 1.46839e+000 |
| 1.360 | 2.94959e+000 | 1.62902e+000 | 2.95174e+000 | 1.54791e+000 | 2.95923e+000 | 1.46945e+000 |

| | | | | | | |
|---|---|---|---|---|---|---|
| 1.370 | 2.95154e+000 | 1.63016e+000 | 2.95372e+000 | 1.54899e+000 | 2.96123e+000 | 1.47047e+000 |
| 1.380 | 2.95344e+000 | 1.63126e+000 | 2.95562e+000 | 1.55002e+000 | 2.96317e+000 | 1.47145e+000 |
| 1.390 | 2.95525e+000 | 1.63233e+000 | 2.95746e+000 | 1.55103e+000 | 2.96502e+000 | 1.47241e+000 |
| 1.400 | 2.95700e+000 | 1.63334e+000 | 2.95923e+000 | 1.55199e+000 | 2.96683e+000 | 1.47332e+000 |
| 1.410 | 2.95868e+000 | 1.63433e+000 | 2.96093e+000 | 1.55292e+000 | 2.96856e+000 | 1.47420e+000 |
| 1.420 | 2.96031e+000 | 1.63528e+000 | 2.96257e+000 | 1.55382e+000 | 2.97022e+000 | 1.47504e+000 |
| 1.430 | 2.96186e+000 | 1.63619e+000 | 2.96414e+000 | 1.55468e+000 | 2.97182e+000 | 1.47586e+000 |
| 1.440 | 2.96337e+000 | 1.63707e+000 | 2.96566e+000 | 1.55551e+000 | 2.97336e+000 | 1.47664e+000 |
| 1.450 | 2.96481e+000 | 1.63791e+000 | 2.96713e+000 | 1.55631e+000 | 2.97485e+000 | 1.47740e+000 |
| 1.460 | 2.96619e+000 | 1.63874e+000 | 2.96852e+000 | 1.55708e+000 | 2.97628e+000 | 1.47813e+000 |
| 1.470 | 2.96752e+000 | 1.63952e+000 | 2.96988e+000 | 1.55782e+000 | 2.97766e+000 | 1.47882e+000 |
| 1.480 | 2.96880e+000 | 1.64027e+000 | 2.97117e+000 | 1.55852e+000 | 2.97898e+000 | 1.47949e+000 |
| 1.490 | 2.97003e+000 | 1.64099e+000 | 2.97242e+000 | 1.55921e+000 | 2.98025e+000 | 1.48013e+000 |
| 1.500 | 2.97121e+000 | 1.64170e+000 | 2.97362e+000 | 1.55987e+000 | 2.98147e+000 | 1.48075e+000 |
| 1.510 | 2.97235e+000 | 1.64236e+000 | 2.97477e+000 | 1.56050e+000 | 2.98265e+000 | 1.48134e+000 |
| 1.520 | 2.97343e+000 | 1.64300e+000 | 2.97587e+000 | 1.56110e+000 | 2.98378e+000 | 1.48191e+000 |
| 1.530 | 2.97447e+000 | 1.64362e+000 | 2.97693e+000 | 1.56168e+000 | 2.98486e+000 | 1.48246e+000 |
| 1.540 | 2.97547e+000 | 1.64422e+000 | 2.97794e+000 | 1.56224e+000 | 2.98590e+000 | 1.48298e+000 |
| 1.550 | 2.97642e+000 | 1.64478e+000 | 2.97892e+000 | 1.56276e+000 | 2.98690e+000 | 1.48348e+000 |
| 1.560 | 2.97734e+000 | 1.64533e+000 | 2.97985e+000 | 1.56328e+000 | 2.98785e+000 | 1.48396e+000 |
| 1.570 | 2.97821e+000 | 1.64586e+000 | 2.98074e+000 | 1.56377e+000 | 2.98877e+000 | 1.48443e+000 |
| 1.580 | 2.97905e+000 | 1.64636e+000 | 2.98160e+000 | 1.56424e+000 | 2.98965e+000 | 1.48487e+000 |
| 1.590 | 2.97986e+000 | 1.64684e+000 | 2.98242e+000 | 1.56469e+000 | 2.99049e+000 | 1.48529e+000 |
| 1.600 | 2.98062e+000 | 1.64729e+000 | 2.98320e+000 | 1.56511e+000 | 2.99130e+000 | 1.48569e+000 |
| 1.610 | 2.98135e+000 | 1.64773e+000 | 2.98394e+000 | 1.56552e+000 | 2.99206e+000 | 1.48607e+000 |
| 1.620 | 2.98204e+000 | 1.64815e+000 | 2.98466e+000 | 1.56592e+000 | 2.99280e+000 | 1.48644e+000 |
| 1.630 | 2.98271e+000 | 1.64855e+000 | 2.98534e+000 | 1.56629e+000 | 2.99350e+000 | 1.48678e+000 |
| 1.640 | 2.98334e+000 | 1.64893e+000 | 2.98599e+000 | 1.56665e+000 | 2.99417e+000 | 1.48711e+000 |
| 1.650 | 2.98394e+000 | 1.64930e+000 | 2.98661e+000 | 1.56698e+000 | 2.99482e+000 | 1.48743e+000 |
| 1.660 | 2.98450e+000 | 1.64964e+000 | 2.98719e+000 | 1.56730e+000 | 2.99542e+000 | 1.48773e+000 |
| 1.670 | 2.98505e+000 | 1.64998e+000 | 2.98775e+000 | 1.56761e+000 | 2.99600e+000 | 1.48802e+000 |
| 1.680 | 2.98556e+000 | 1.65030e+000 | 2.98828e+000 | 1.56791e+000 | 2.99655e+000 | 1.48829e+000 |
| 1.690 | 2.98605e+000 | 1.65059e+000 | 2.98878e+000 | 1.56818e+000 | 2.99708e+000 | 1.48855e+000 |
| 1.700 | 2.98652e+000 | 1.65087e+000 | 2.98927e+000 | 1.56844e+000 | 2.99759e+000 | 1.48879e+000 |
| 1.710 | 2.98695e+000 | 1.65114e+000 | 2.98972e+000 | 1.56869e+000 | 2.99806e+000 | 1.48901e+000 |
| 1.720 | 2.98736e+000 | 1.65140e+000 | 2.99015e+000 | 1.56892e+000 | 2.99851e+000 | 1.48923e+000 |
| 1.730 | 2.98774e+000 | 1.65164e+000 | 2.99054e+000 | 1.56914e+000 | 2.99893e+000 | 1.48943e+000 |
| 1.740 | 2.98811e+000 | 1.65186e+000 | 2.99092e+000 | 1.56935e+000 | 2.99933e+000 | 1.48963e+000 |
| 1.750 | 2.98845e+000 | 1.65208e+000 | 2.99128e+000 | 1.56955e+000 | 2.99970e+000 | 1.48981e+000 |
| 1.760 | 2.98877e+000 | 1.65228e+000 | 2.99161e+000 | 1.56973e+000 | 3.00006e+000 | 1.48997e+000 |
| 1.770 | 2.98907e+000 | 1.65246e+000 | 2.99193e+000 | 1.56990e+000 | 3.00040e+000 | 1.49012e+000 |
| 1.780 | 2.98934e+000 | 1.65264e+000 | 2.99222e+000 | 1.57006e+000 | 3.00071e+000 | 1.49027e+000 |
| 1.790 | 2.98959e+000 | 1.65280e+000 | 2.99249e+000 | 1.57020e+000 | 3.00100e+000 | 1.49040e+000 |
| 1.800 | 2.98984e+000 | 1.65296e+000 | 2.99274e+000 | 1.57034e+000 | 3.00127e+000 | 1.49053e+000 |
| 1.810 | 2.99005e+000 | 1.65310e+000 | 2.99297e+000 | 1.57047e+000 | 3.00153e+000 | 1.49064e+000 |
| 1.820 | 2.99025e+000 | 1.65324e+000 | 2.99319e+000 | 1.57059e+000 | 3.00177e+000 | 1.49075e+000 |
| 1.830 | 2.99044e+000 | 1.65336e+000 | 2.99339e+000 | 1.57070e+000 | 3.00199e+000 | 1.49084e+000 |
| 1.840 | 2.99061e+000 | 1.65347e+000 | 2.99358e+000 | 1.57080e+000 | 3.00219e+000 | 1.49093e+000 |
| 1.850 | 2.99077e+000 | 1.65357e+000 | 2.99375e+000 | 1.57088e+000 | 3.00238e+000 | 1.49101e+000 |
| 1.860 | 2.99090e+000 | 1.65366e+000 | 2.99390e+000 | 1.57097e+000 | 3.00255e+000 | 1.49108e+000 |
| 1.870 | 2.99102e+000 | 1.65375e+000 | 2.99404e+000 | 1.57104e+000 | 3.00271e+000 | 1.49114e+000 |
| 1.880 | 2.99112e+000 | 1.65383e+000 | 2.99415e+000 | 1.57110e+000 | 3.00285e+000 | 1.49119e+000 |
| 1.890 | 2.99120e+000 | 1.65389e+000 | 2.99425e+000 | 1.57115e+000 | 3.00297e+000 | 1.49124e+000 |
| 1.900 | 2.99128e+000 | 1.65395e+000 | 2.99434e+000 | 1.57120e+000 | 3.00307e+000 | 1.49127e+000 |
| 1.910 | 2.99134e+000 | 1.65399e+000 | 2.99442e+000 | 1.57123e+000 | 3.00317e+000 | 1.49130e+000 |
| 1.920 | 2.99138e+000 | 1.65403e+000 | 2.99447e+000 | 1.57126e+000 | 3.00325e+000 | 1.49132e+000 |
| 1.930 | 2.99142e+000 | 1.65407e+000 | 2.99453e+000 | 1.57129e+000 | 3.00332e+000 | 1.49134e+000 |
| 1.940 | 2.99144e+000 | 1.65410e+000 | 2.99457e+000 | 1.57131e+000 | 3.00337e+000 | 1.49135e+000 |
| 1.950 | 2.99145e+000 | 1.65412e+000 | 2.99459e+000 | 1.57132e+000 | 3.00342e+000 | 1.49136e+000 |
| 1.960 | 2.99147e+000 | 1.65414e+000 | 2.99462e+000 | 1.57133e+000 | 3.00346e+000 | 1.49135e+000 |
| 1.970 | 2.99146e+000 | 1.65414e+000 | 2.99462e+000 | 1.57132e+000 | 3.00348e+000 | 1.49135e+000 |
| 1.980 | 2.99143e+000 | 1.65414e+000 | 2.99461e+000 | 1.57132e+000 | 3.00349e+000 | 1.49133e+000 |
| 1.990 | 2.99139e+000 | 1.65413e+000 | 2.99458e+000 | 1.57130e+000 | 3.00348e+000 | 1.49131e+000 |
| 2.000 | 2.99135e+000 | 1.65412e+000 | 2.99456e+000 | 1.57128e+000 | 3.00348e+000 | 1.49128e+000 |
| 2.010 | 2.99129e+000 | 1.65410e+000 | 2.99452e+000 | 1.57125e+000 | 3.00345e+000 | 1.49125e+000 |
| 2.020 | 2.99123e+000 | 1.65408e+000 | 2.99447e+000 | 1.57122e+000 | 3.00343e+000 | 1.49121e+000 |
| 2.030 | 2.99115e+000 | 1.65404e+000 | 2.99441e+000 | 1.57118e+000 | 3.00338e+000 | 1.49117e+000 |
| 2.040 | 2.99108e+000 | 1.65401e+000 | 2.99434e+000 | 1.57114e+000 | 3.00333e+000 | 1.49112e+000 |
| 2.050 | 2.99099e+000 | 1.65396e+000 | 2.99427e+000 | 1.57109e+000 | 3.00327e+000 | 1.49107e+000 |
| 2.060 | 2.99089e+000 | 1.65392e+000 | 2.99418e+000 | 1.57104e+000 | 3.00321e+000 | 1.49101e+000 |
| 2.070 | 2.99078e+000 | 1.65387e+000 | 2.99409e+000 | 1.57099e+000 | 3.00313e+000 | 1.49095e+000 |
| 2.080 | 2.99067e+000 | 1.65381e+000 | 2.99399e+000 | 1.57092e+000 | 3.00305e+000 | 1.49089e+000 |
| 2.090 | 2.99054e+000 | 1.65375e+000 | 2.99387e+000 | 1.57086e+000 | 3.00295e+000 | 1.49082e+000 |
| 2.100 | 2.99040e+000 | 1.65369e+000 | 2.99375e+000 | 1.57078e+000 | 3.00285e+000 | 1.49075e+000 |
| 2.110 | 2.99027e+000 | 1.65362e+000 | 2.99363e+000 | 1.57071e+000 | 3.00274e+000 | 1.49067e+000 |
| 2.120 | 2.99013e+000 | 1.65356e+000 | 2.99351e+000 | 1.57064e+000 | 3.00263e+000 | 1.49059e+000 |
| 2.130 | 2.98999e+000 | 1.65348e+000 | 2.99338e+000 | 1.57056e+000 | 3.00252e+000 | 1.49051e+000 |
| 2.140 | 2.98983e+000 | 1.65339e+000 | 2.99323e+000 | 1.57047e+000 | 3.00239e+000 | 1.49042e+000 |
| 2.150 | 2.98966e+000 | 1.65330e+000 | 2.99308e+000 | 1.57037e+000 | 3.00225e+000 | 1.49032e+000 |
| 2.160 | 2.98949e+000 | 1.65322e+000 | 2.99292e+000 | 1.57028e+000 | 3.00212e+000 | 1.49023e+000 |
| 2.170 | 2.98931e+000 | 1.65312e+000 | 2.99276e+000 | 1.57019e+000 | 3.00197e+000 | 1.49013e+000 |
| 2.180 | 2.98913e+000 | 1.65303e+000 | 2.99259e+000 | 1.57010e+000 | 3.00182e+000 | 1.49003e+000 |
| 2.190 | 2.98895e+000 | 1.65293e+000 | 2.99241e+000 | 1.56999e+000 | 3.00166e+000 | 1.48993e+000 |

| | | | | | | |
|---|---|---|---|---|---|---|
| 2.200 | 2.98876e+000 | 1.65282e+000 | 2.99223e+000 | 1.56988e+000 | 3.00150e+000 | 1.48982e+000 |
| 2.210 | 2.98855e+000 | 1.65271e+000 | 2.99204e+000 | 1.56977e+000 | 3.00133e+000 | 1.48971e+000 |
| 2.220 | 2.98835e+000 | 1.65261e+000 | 2.99186e+000 | 1.56966e+000 | 3.00116e+000 | 1.48959e+000 |
| 2.230 | 2.98815e+000 | 1.65249e+000 | 2.99167e+000 | 1.56954e+000 | 3.00098e+000 | 1.48947e+000 |
| 2.240 | 2.98794e+000 | 1.65238e+000 | 2.99147e+000 | 1.56943e+000 | 3.00081e+000 | 1.48936e+000 |
| 2.250 | 2.98772e+000 | 1.65227e+000 | 2.99126e+000 | 1.56931e+000 | 3.00060e+000 | 1.48924e+000 |
| 2.260 | 2.98750e+000 | 1.65214e+000 | 2.99105e+000 | 1.56918e+000 | 3.00041e+000 | 1.48911e+000 |
| 2.270 | 2.98727e+000 | 1.65202e+000 | 2.99084e+000 | 1.56906e+000 | 3.00021e+000 | 1.48899e+000 |
| 2.280 | 2.98705e+000 | 1.65190e+000 | 2.99063e+000 | 1.56894e+000 | 3.00002e+000 | 1.48887e+000 |
| 2.290 | 2.98682e+000 | 1.65178e+000 | 2.99041e+000 | 1.56881e+000 | 2.99982e+000 | 1.48874e+000 |
| 2.300 | 2.98659e+000 | 1.65164e+000 | 2.99019e+000 | 1.56867e+000 | 2.99962e+000 | 1.48860e+000 |
| 2.310 | 2.98635e+000 | 1.65151e+000 | 2.98997e+000 | 1.56854e+000 | 2.99941e+000 | 1.48847e+000 |
| 2.320 | 2.98610e+000 | 1.65138e+000 | 2.98973e+000 | 1.56841e+000 | 2.99918e+000 | 1.48834e+000 |
| 2.330 | 2.98584e+000 | 1.65123e+000 | 2.98948e+000 | 1.56826e+000 | 2.99895e+000 | 1.48819e+000 |
| 2.340 | 2.98559e+000 | 1.65109e+000 | 2.98924e+000 | 1.56812e+000 | 2.99872e+000 | 1.48805e+000 |
| 2.350 | 2.98533e+000 | 1.65095e+000 | 2.98900e+000 | 1.56798e+000 | 2.99850e+000 | 1.48791e+000 |
| 2.360 | 2.98508e+000 | 1.65081e+000 | 2.98876e+000 | 1.56784e+000 | 2.99827e+000 | 1.48777e+000 |
| 2.370 | 2.98482e+000 | 1.65067e+000 | 2.98851e+000 | 1.56769e+000 | 2.99804e+000 | 1.48763e+000 |
| 2.380 | 2.98456e+000 | 1.65052e+000 | 2.98826e+000 | 1.56754e+000 | 2.99780e+000 | 1.48748e+000 |
| 2.390 | 2.98429e+000 | 1.65037e+000 | 2.98801e+000 | 1.56739e+000 | 2.99756e+000 | 1.48732e+000 |
| 2.400 | 2.98403e+000 | 1.65022e+000 | 2.98776e+000 | 1.56724e+000 | 2.99733e+000 | 1.48717e+000 |
| 2.410 | 2.98377e+000 | 1.65007e+000 | 2.98751e+000 | 1.56709e+000 | 2.99710e+000 | 1.48703e+000 |
| 2.420 | 2.98350e+000 | 1.64992e+000 | 2.98725e+000 | 1.56694e+000 | 2.99685e+000 | 1.48688e+000 |
| 2.430 | 2.98323e+000 | 1.64977e+000 | 2.98699e+000 | 1.56679e+000 | 2.99660e+000 | 1.48673e+000 |
| 2.440 | 2.98295e+000 | 1.64962e+000 | 2.98672e+000 | 1.56664e+000 | 2.99636e+000 | 1.48658e+000 |
| 2.450 | 2.98268e+000 | 1.64947e+000 | 2.98647e+000 | 1.56649e+000 | 2.99611e+000 | 1.48643e+000 |
| 2.460 | 2.98240e+000 | 1.64930e+000 | 2.98619e+000 | 1.56632e+000 | 2.99586e+000 | 1.48627e+000 |
| 2.470 | 2.98211e+000 | 1.64914e+000 | 2.98592e+000 | 1.56617e+000 | 2.99560e+000 | 1.48611e+000 |
| 2.480 | 2.98184e+000 | 1.64899e+000 | 2.98565e+000 | 1.56601e+000 | 2.99534e+000 | 1.48595e+000 |
| 2.490 | 2.98155e+000 | 1.64883e+000 | 2.98538e+000 | 1.56585e+000 | 2.99508e+000 | 1.48580e+000 |
| 2.500 | 2.98127e+000 | 1.64866e+000 | 2.98511e+000 | 1.56569e+000 | 2.99483e+000 | 1.48564e+000 |
| 2.550 | 2.97980e+000 | 1.64783e+000 | 2.98370e+000 | 1.56485e+000 | 2.99348e+000 | 1.48481e+000 |
| 2.600 | 2.97831e+000 | 1.64697e+000 | 2.98226e+000 | 1.56400e+000 | 2.99211e+000 | 1.48397e+000 |
| 2.650 | 2.97680e+000 | 1.64611e+000 | 2.98080e+000 | 1.56314e+000 | 2.99071e+000 | 1.48313e+000 |
| 2.700 | 2.97528e+000 | 1.64524e+000 | 2.97933e+000 | 1.56229e+000 | 2.98931e+000 | 1.48228e+000 |
| 2.750 | 2.97376e+000 | 1.64435e+000 | 2.97787e+000 | 1.56140e+000 | 2.98792e+000 | 1.48141e+000 |
| 2.800 | 2.97223e+000 | 1.64346e+000 | 2.97639e+000 | 1.56052e+000 | 2.98649e+000 | 1.48055e+000 |
| 2.850 | 2.97068e+000 | 1.64258e+000 | 2.97487e+000 | 1.55964e+000 | 2.98504e+000 | 1.47968e+000 |
| 2.900 | 2.96912e+000 | 1.64166e+000 | 2.97338e+000 | 1.55874e+000 | 2.98360e+000 | 1.47880e+000 |
| 2.950 | 2.96758e+000 | 1.64076e+000 | 2.97189e+000 | 1.55785e+000 | 2.98216e+000 | 1.47792e+000 |
| 3.000 | 2.96608e+000 | 1.63988e+000 | 2.97042e+000 | 1.55698e+000 | 2.98075e+000 | 1.47707e+000 |
| 3.050 | 2.96459e+000 | 1.63901e+000 | 2.96898e+000 | 1.55612e+000 | 2.97937e+000 | 1.47623e+000 |
| 3.100 | 2.96309e+000 | 1.63813e+000 | 2.96752e+000 | 1.55525e+000 | 2.97797e+000 | 1.47537e+000 |
| 3.150 | 2.96161e+000 | 1.63725e+000 | 2.96608e+000 | 1.55438e+000 | 2.97658e+000 | 1.47452e+000 |
| 3.200 | 2.96014e+000 | 1.63638e+000 | 2.96466e+000 | 1.55353e+000 | 2.97520e+000 | 1.47368e+000 |
| 3.250 | 2.95866e+000 | 1.63551e+000 | 2.96321e+000 | 1.55267e+000 | 2.97381e+000 | 1.47284e+000 |
| 3.300 | 2.95722e+000 | 1.63466e+000 | 2.96182e+000 | 1.55183e+000 | 2.97246e+000 | 1.47202e+000 |
| 3.350 | 2.95581e+000 | 1.63382e+000 | 2.96045e+000 | 1.55101e+000 | 2.97113e+000 | 1.47121e+000 |
| 3.400 | 2.95444e+000 | 1.63301e+000 | 2.95912e+000 | 1.55020e+000 | 2.96985e+000 | 1.47042e+000 |
| 3.450 | 2.95308e+000 | 1.63220e+000 | 2.95779e+000 | 1.54941e+000 | 2.96857e+000 | 1.46964e+000 |
| 3.500 | 2.95174e+000 | 1.63139e+000 | 2.95648e+000 | 1.54862e+000 | 2.96730e+000 | 1.46887e+000 |
| 3.550 | 2.95039e+000 | 1.63059e+000 | 2.95518e+000 | 1.54783e+000 | 2.96605e+000 | 1.46810e+000 |
| 3.600 | 2.94907e+000 | 1.62980e+000 | 2.95389e+000 | 1.54705e+000 | 2.96480e+000 | 1.46733e+000 |
| 3.650 | 2.94778e+000 | 1.62903e+000 | 2.95263e+000 | 1.54630e+000 | 2.96358e+000 | 1.46660e+000 |
| 3.700 | 2.94649e+000 | 1.62825e+000 | 2.95138e+000 | 1.54553e+000 | 2.96237e+000 | 1.46584e+000 |
| 3.750 | 2.94523e+000 | 1.62749e+000 | 2.95015e+000 | 1.54477e+000 | 2.96118e+000 | 1.46511e+000 |
| 3.800 | 2.94401e+000 | 1.62677e+000 | 2.94896e+000 | 1.54406e+000 | 2.96003e+000 | 1.46441e+000 |
| 3.850 | 2.94283e+000 | 1.62605e+000 | 2.94781e+000 | 1.54336e+000 | 2.95892e+000 | 1.46372e+000 |
| 3.900 | 2.94166e+000 | 1.62535e+000 | 2.94667e+000 | 1.54267e+000 | 2.95782e+000 | 1.46304e+000 |
| 3.950 | 2.94049e+000 | 1.62464e+000 | 2.94553e+000 | 1.54197e+000 | 2.95671e+000 | 1.46236e+000 |
| 4.000 | 2.93932e+000 | 1.62393e+000 | 2.94440e+000 | 1.54128e+000 | 2.95562e+000 | 1.46168e+000 |
| 4.050 | 2.93818e+000 | 1.62324e+000 | 2.94329e+000 | 1.54060e+000 | 2.95454e+000 | 1.46102e+000 |
| 4.100 | 2.93708e+000 | 1.62257e+000 | 2.94221e+000 | 1.53994e+000 | 2.95350e+000 | 1.46037e+000 |
| 4.150 | 2.93597e+000 | 1.62190e+000 | 2.94113e+000 | 1.53928e+000 | 2.95245e+000 | 1.45972e+000 |
| 4.200 | 2.93489e+000 | 1.62125e+000 | 2.94008e+000 | 1.53863e+000 | 2.95143e+000 | 1.45910e+000 |
| 4.250 | 2.93384e+000 | 1.62061e+000 | 2.93906e+000 | 1.53800e+000 | 2.95044e+000 | 1.45848e+000 |
| 4.300 | 2.93282e+000 | 1.61999e+000 | 2.93806e+000 | 1.53740e+000 | 2.94949e+000 | 1.45789e+000 |
| 4.350 | 2.93182e+000 | 1.61937e+000 | 2.93709e+000 | 1.53679e+000 | 2.94854e+000 | 1.45730e+000 |
| 4.400 | 2.93082e+000 | 1.61878e+000 | 2.93612e+000 | 1.53620e+000 | 2.94761e+000 | 1.45672e+000 |
| 4.450 | 2.92986e+000 | 1.61817e+000 | 2.93518e+000 | 1.53561e+000 | 2.94669e+000 | 1.45613e+000 |
| 4.500 | 2.92888e+000 | 1.61758e+000 | 2.93422e+000 | 1.53503e+000 | 2.94576e+000 | 1.45557e+000 |
| 4.550 | 2.92791e+000 | 1.61699e+000 | 2.93327e+000 | 1.53445e+000 | 2.94484e+000 | 1.45500e+000 |
| 4.600 | 2.92698e+000 | 1.61641e+000 | 2.93237e+000 | 1.53388e+000 | 2.94398e+000 | 1.45444e+000 |
| 4.650 | 2.92606e+000 | 1.61585e+000 | 2.93148e+000 | 1.53332e+000 | 2.94310e+000 | 1.45389e+000 |
| 4.700 | 2.92515e+000 | 1.61530e+000 | 2.93058e+000 | 1.53279e+000 | 2.94224e+000 | 1.45337e+000 |
| 4.750 | 2.92428e+000 | 1.61477e+000 | 2.92974e+000 | 1.53226e+000 | 2.94143e+000 | 1.45286e+000 |
| 4.800 | 2.92341e+000 | 1.61423e+000 | 2.92890e+000 | 1.53173e+000 | 2.94061e+000 | 1.45233e+000 |
| 4.850 | 2.92256e+000 | 1.61370e+000 | 2.92808e+000 | 1.53121e+000 | 2.93982e+000 | 1.45183e+000 |
| 4.900 | 2.92172e+000 | 1.61319e+000 | 2.92725e+000 | 1.53071e+000 | 2.93901e+000 | 1.45134e+000 |
| 4.950 | 2.92089e+000 | 1.61269e+000 | 2.92644e+000 | 1.53021e+000 | 2.93824e+000 | 1.45085e+000 |
| 5.000 | 2.92006e+000 | 1.61216e+000 | 2.92563e+000 | 1.52970e+000 | 2.93745e+000 | 1.45035e+000 |
| 5.050 | 2.91926e+000 | 1.61166e+000 | 2.92485e+000 | 1.52921e+000 | 2.93669e+000 | 1.44987e+000 |
| 5.100 | 2.91847e+000 | 1.61118e+000 | 2.92408e+000 | 1.52873e+000 | 2.93595e+000 | 1.44940e+000 |

| | | | | | | |
|---|---|---|---|---|---|---|
| 5.150 | 2.91770e+000 | 1.61070e+000 | 2.92333e+000 | 1.52826e+000 | 2.93522e+000 | 1.44894e+000 |
| 5.200 | 2.91694e+000 | 1.61023e+000 | 2.92259e+000 | 1.52780e+000 | 2.93451e+000 | 1.44849e+000 |
| 5.250 | 2.91620e+000 | 1.60977e+000 | 2.92187e+000 | 1.52735e+000 | 2.93381e+000 | 1.44805e+000 |
| 5.300 | 2.91547e+000 | 1.60933e+000 | 2.92116e+000 | 1.52691e+000 | 2.93312e+000 | 1.44761e+000 |
| 5.350 | 2.91474e+000 | 1.60887e+000 | 2.92045e+000 | 1.52646e+000 | 2.93243e+000 | 1.44718e+000 |
| 5.400 | 2.91403e+000 | 1.60843e+000 | 2.91976e+000 | 1.52603e+000 | 2.93176e+000 | 1.44675e+000 |
| 5.450 | 2.91334e+000 | 1.60799e+000 | 2.91908e+000 | 1.52560e+000 | 2.93111e+000 | 1.44633e+000 |
| 5.500 | 2.91265e+000 | 1.60757e+000 | 2.91841e+000 | 1.52518e+000 | 2.93046e+000 | 1.44592e+000 |
| 5.550 | 2.91197e+000 | 1.60715e+000 | 2.91775e+000 | 1.52477e+000 | 2.92982e+000 | 1.44552e+000 |
| 5.600 | 2.91131e+000 | 1.60673e+000 | 2.91710e+000 | 1.52436e+000 | 2.92920e+000 | 1.44512e+000 |
| 5.650 | 2.91066e+000 | 1.60633e+000 | 2.91647e+000 | 1.52396e+000 | 2.92858e+000 | 1.44473e+000 |
| 5.700 | 2.91002e+000 | 1.60593e+000 | 2.91585e+000 | 1.52357e+000 | 2.92798e+000 | 1.44434e+000 |
| 5.750 | 2.90938e+000 | 1.60553e+000 | 2.91523e+000 | 1.52317e+000 | 2.92738e+000 | 1.44396e+000 |
| 5.800 | 2.90875e+000 | 1.60514e+000 | 2.91462e+000 | 1.52279e+000 | 2.92679e+000 | 1.44358e+000 |
| 5.850 | 2.90813e+000 | 1.60476e+000 | 2.91402e+000 | 1.52241e+000 | 2.92621e+000 | 1.44321e+000 |
| 5.900 | 2.90754e+000 | 1.60438e+000 | 2.91343e+000 | 1.52204e+000 | 2.92564e+000 | 1.44285e+000 |
| 5.950 | 2.90695e+000 | 1.60401e+000 | 2.91286e+000 | 1.52167e+000 | 2.92509e+000 | 1.44249e+000 |
| 6.000 | 2.90636e+000 | 1.60364e+000 | 2.91229e+000 | 1.52132e+000 | 2.92454e+000 | 1.44214e+000 |
| 6.050 | 2.90578e+000 | 1.60328e+000 | 2.91172e+000 | 1.52096e+000 | 2.92399e+000 | 1.44179e+000 |
| 6.100 | 2.90521e+000 | 1.60293e+000 | 2.91117e+000 | 1.52061e+000 | 2.92346e+000 | 1.44144e+000 |
| 6.150 | 2.90466e+000 | 1.60257e+000 | 2.91063e+000 | 1.52026e+000 | 2.92293e+000 | 1.44110e+000 |
| 6.200 | 2.90410e+000 | 1.60223e+000 | 2.91009e+000 | 1.51992e+000 | 2.92241e+000 | 1.44077e+000 |
| 6.250 | 2.90356e+000 | 1.60189e+000 | 2.90957e+000 | 1.51959e+000 | 2.92190e+000 | 1.44044e+000 |
| 6.300 | 2.90302e+000 | 1.60155e+000 | 2.90904e+000 | 1.51926e+000 | 2.92139e+000 | 1.44012e+000 |
| 6.350 | 2.90250e+000 | 1.60122e+000 | 2.90853e+000 | 1.51893e+000 | 2.92091e+000 | 1.43980e+000 |
| 6.400 | 2.90198e+000 | 1.60090e+000 | 2.90803e+000 | 1.51861e+000 | 2.92041e+000 | 1.43948e+000 |
| 6.450 | 2.90147e+000 | 1.60058e+000 | 2.90753e+000 | 1.51829e+000 | 2.91993e+000 | 1.43918e+000 |
| 6.500 | 2.90097e+000 | 1.60026e+000 | 2.90704e+000 | 1.51798e+000 | 2.91946e+000 | 1.43887e+000 |
| 6.550 | 2.90048e+000 | 1.59995e+000 | 2.90657e+000 | 1.51767e+000 | 2.91900e+000 | 1.43857e+000 |
| 6.600 | 2.89998e+000 | 1.59963e+000 | 2.90608e+000 | 1.51737e+000 | 2.91853e+000 | 1.43826e+000 |
| 6.650 | 2.89950e+000 | 1.59933e+000 | 2.90561e+000 | 1.51707e+000 | 2.91808e+000 | 1.43797e+000 |
| 6.700 | 2.89903e+000 | 1.59903e+000 | 2.90515e+000 | 1.51677e+000 | 2.91763e+000 | 1.43768e+000 |
| 6.750 | 2.89856e+000 | 1.59874e+000 | 2.90469e+000 | 1.51649e+000 | 2.91719e+000 | 1.43740e+000 |
| 6.800 | 2.89810e+000 | 1.59845e+000 | 2.90425e+000 | 1.51620e+000 | 2.91676e+000 | 1.43712e+000 |
| 6.850 | 2.89765e+000 | 1.59816e+000 | 2.90381e+000 | 1.51591e+000 | 2.91634e+000 | 1.43684e+000 |
| 6.900 | 2.89718e+000 | 1.59787e+000 | 2.90336e+000 | 1.51563e+000 | 2.91590e+000 | 1.43656e+000 |
| 6.950 | 2.89673e+000 | 1.59759e+000 | 2.90292e+000 | 1.51535e+000 | 2.91548e+000 | 1.43629e+000 |
| 7.000 | 2.89631e+000 | 1.59731e+000 | 2.90250e+000 | 1.51508e+000 | 2.91507e+000 | 1.43602e+000 |
| 7.050 | 2.89587e+000 | 1.59703e+000 | 2.90208e+000 | 1.51481e+000 | 2.91467e+000 | 1.43575e+000 |
| 7.100 | 2.89545e+000 | 1.59676e+000 | 2.90167e+000 | 1.51454e+000 | 2.91427e+000 | 1.43549e+000 |
| 7.150 | 2.89503e+000 | 1.59650e+000 | 2.90126e+000 | 1.51428e+000 | 2.91388e+000 | 1.43524e+000 |
| 7.200 | 2.89463e+000 | 1.59625e+000 | 2.90087e+000 | 1.51403e+000 | 2.91349e+000 | 1.43499e+000 |
| 7.250 | 2.89422e+000 | 1.59599e+000 | 2.90047e+000 | 1.51377e+000 | 2.91311e+000 | 1.43474e+000 |
| 7.300 | 2.89382e+000 | 1.59574e+000 | 2.90008e+000 | 1.51353e+000 | 2.91274e+000 | 1.43450e+000 |
| 7.350 | 2.89342e+000 | 1.59548e+000 | 2.89969e+000 | 1.51328e+000 | 2.91236e+000 | 1.43425e+000 |
| 7.400 | 2.89303e+000 | 1.59523e+000 | 2.89931e+000 | 1.51303e+000 | 2.91199e+000 | 1.43401e+000 |
| 7.450 | 2.89264e+000 | 1.59497e+000 | 2.89894e+000 | 1.51278e+000 | 2.91162e+000 | 1.43376e+000 |
| 7.500 | 2.89225e+000 | 1.59473e+000 | 2.89856e+000 | 1.51254e+000 | 2.91126e+000 | 1.43353e+000 |
| 7.550 | 2.89186e+000 | 1.59449e+000 | 2.89818e+000 | 1.51229e+000 | 2.91090e+000 | 1.43329e+000 |
| 7.600 | 2.89150e+000 | 1.59425e+000 | 2.89782e+000 | 1.51206e+000 | 2.91055e+000 | 1.43306e+000 |
| 7.650 | 2.89112e+000 | 1.59402e+000 | 2.89745e+000 | 1.51183e+000 | 2.91020e+000 | 1.43283e+000 |
| 7.700 | 2.89075e+000 | 1.59378e+000 | 2.89710e+000 | 1.51160e+000 | 2.90985e+000 | 1.43261e+000 |
| 7.750 | 2.89040e+000 | 1.59356e+000 | 2.89676e+000 | 1.51138e+000 | 2.90952e+000 | 1.43239e+000 |
| 7.800 | 2.89005e+000 | 1.59333e+000 | 2.89642e+000 | 1.51116e+000 | 2.90919e+000 | 1.43217e+000 |
| 7.850 | 2.88971e+000 | 1.59312e+000 | 2.89608e+000 | 1.51094e+000 | 2.90887e+000 | 1.43196e+000 |
| 7.900 | 2.88936e+000 | 1.59289e+000 | 2.89575e+000 | 1.51072e+000 | 2.90855e+000 | 1.43175e+000 |
| 7.950 | 2.88903e+000 | 1.59268e+000 | 2.89543e+000 | 1.51051e+000 | 2.90824e+000 | 1.43154e+000 |
| 8.000 | 2.88870e+000 | 1.59246e+000 | 2.89511e+000 | 1.51030e+000 | 2.90792e+000 | 1.43133e+000 |
| 8.050 | 2.88837e+000 | 1.59225e+000 | 2.89478e+000 | 1.51009e+000 | 2.90762e+000 | 1.43113e+000 |
| 8.100 | 2.88803e+000 | 1.59204e+000 | 2.89446e+000 | 1.50988e+000 | 2.90730e+000 | 1.43092e+000 |
| 8.150 | 2.88771e+000 | 1.59184e+000 | 2.89414e+000 | 1.50968e+000 | 2.90700e+000 | 1.43072e+000 |
| 8.200 | 2.88739e+000 | 1.59164e+000 | 2.89383e+000 | 1.50948e+000 | 2.90670e+000 | 1.43053e+000 |
| 8.250 | 2.88707e+000 | 1.59143e+000 | 2.89352e+000 | 1.50927e+000 | 2.90639e+000 | 1.43033e+000 |
| 8.300 | 2.88675e+000 | 1.59122e+000 | 2.89321e+000 | 1.50907e+000 | 2.90609e+000 | 1.43013e+000 |
| 8.350 | 2.88643e+000 | 1.59102e+000 | 2.89290e+000 | 1.50887e+000 | 2.90580e+000 | 1.42993e+000 |
| 8.400 | 2.88612e+000 | 1.59082e+000 | 2.89260e+000 | 1.50868e+000 | 2.90551e+000 | 1.42974e+000 |
| 8.450 | 2.88582e+000 | 1.59062e+000 | 2.89230e+000 | 1.50848e+000 | 2.90522e+000 | 1.42955e+000 |
| 8.500 | 2.88551e+000 | 1.59043e+000 | 2.89201e+000 | 1.50829e+000 | 2.90494e+000 | 1.42936e+000 |
| 8.550 | 2.88522e+000 | 1.59024e+000 | 2.89173e+000 | 1.50810e+000 | 2.90467e+000 | 1.42917e+000 |
| 8.600 | 2.88495e+000 | 1.59006e+000 | 2.89145e+000 | 1.50793e+000 | 2.90440e+000 | 1.42900e+000 |
| 8.650 | 2.88467e+000 | 1.58988e+000 | 2.89118e+000 | 1.50775e+000 | 2.90413e+000 | 1.42883e+000 |
| 8.700 | 2.88438e+000 | 1.58970e+000 | 2.89091e+000 | 1.50757e+000 | 2.90387e+000 | 1.42866e+000 |
| 8.750 | 2.88411e+000 | 1.58953e+000 | 2.89065e+000 | 1.50740e+000 | 2.90362e+000 | 1.42848e+000 |
| 8.800 | 2.88383e+000 | 1.58935e+000 | 2.89038e+000 | 1.50723e+000 | 2.90336e+000 | 1.42831e+000 |
| 8.850 | 2.88357e+000 | 1.58918e+000 | 2.89012e+000 | 1.50705e+000 | 2.90311e+000 | 1.42814e+000 |
| 8.900 | 2.88330e+000 | 1.58900e+000 | 2.88986e+000 | 1.50688e+000 | 2.90286e+000 | 1.42797e+000 |
| 8.950 | 2.88303e+000 | 1.58882e+000 | 2.88960e+000 | 1.50671e+000 | 2.90261e+000 | 1.42780e+000 |
| 9.000 | 2.88276e+000 | 1.58865e+000 | 2.88933e+000 | 1.50653e+000 | 2.90235e+000 | 1.42763e+000 |
| 9.050 | 2.88250e+000 | 1.58848e+000 | 2.88908e+000 | 1.50637e+000 | 2.90211e+000 | 1.42747e+000 |
| 9.100 | 2.88224e+000 | 1.58832e+000 | 2.88883e+000 | 1.50621e+000 | 2.90187e+000 | 1.42731e+000 |
| 9.150 | 2.88198e+000 | 1.58815e+000 | 2.88857e+000 | 1.50604e+000 | 2.90163e+000 | 1.42715e+000 |
| 9.200 | 2.88172e+000 | 1.58798e+000 | 2.88832e+000 | 1.50587e+000 | 2.90138e+000 | 1.42698e+000 |
| 9.250 | 2.88146e+000 | 1.58782e+000 | 2.88807e+000 | 1.50571e+000 | 2.90113e+000 | 1.42683e+000 |

| | | | | | | |
|---|---|---|---|---|---|---|
| 9.300 | 2.88120e+000 | 1.58765e+000 | 2.88782e+000 | 1.50555e+000 | 2.90090e+000 | 1.42667e+000 |
| 9.350 | 2.88095e+000 | 1.58749e+000 | 2.88757e+000 | 1.50539e+000 | 2.90066e+000 | 1.42651e+000 |
| 9.400 | 2.88071e+000 | 1.58733e+000 | 2.88733e+000 | 1.50523e+000 | 2.90043e+000 | 1.42636e+000 |
| 9.450 | 2.88047e+000 | 1.58717e+000 | 2.88710e+000 | 1.50508e+000 | 2.90020e+000 | 1.42620e+000 |
| 9.500 | 2.88023e+000 | 1.58702e+000 | 2.88688e+000 | 1.50493e+000 | 2.89998e+000 | 1.42605e+000 |
| 9.550 | 2.88000e+000 | 1.58687e+000 | 2.88665e+000 | 1.50478e+000 | 2.89977e+000 | 1.42591e+000 |
| 9.600 | 2.87978e+000 | 1.58673e+000 | 2.88644e+000 | 1.50464e+000 | 2.89956e+000 | 1.42577e+000 |
| 9.650 | 2.87955e+000 | 1.58658e+000 | 2.88622e+000 | 1.50449e+000 | 2.89935e+000 | 1.42563e+000 |
| 9.700 | 2.87934e+000 | 1.58644e+000 | 2.88601e+000 | 1.50436e+000 | 2.89915e+000 | 1.42550e+000 |
| 9.750 | 2.87912e+000 | 1.58630e+000 | 2.88580e+000 | 1.50421e+000 | 2.89895e+000 | 1.42535e+000 |
| 9.800 | 2.87891e+000 | 1.58616e+000 | 2.88558e+000 | 1.50408e+000 | 2.89873e+000 | 1.42522e+000 |
| 9.850 | 2.87868e+000 | 1.58601e+000 | 2.88537e+000 | 1.50393e+000 | 2.89853e+000 | 1.42508e+000 |
| 9.900 | 2.87847e+000 | 1.58588e+000 | 2.88516e+000 | 1.50380e+000 | 2.89833e+000 | 1.42495e+000 |
| 9.950 | 2.87825e+000 | 1.58573e+000 | 2.88496e+000 | 1.50366e+000 | 2.89814e+000 | 1.42480e+000 |
| 10.000 | 2.87804e+000 | 1.58560e+000 | 2.88474e+000 | 1.50352e+000 | 2.89793e+000 | 1.42467e+000 |

TABLE II: The antineutrino cross sections.

| $E_\nu$ (GeV) | total | neutrons | total | neutrons | total | neutrons |
|---|---|---|---|---|---|---|
| | $g_A^s = -0.03$ | | $g_A^s = -0.08$ | | $g_A^s = -0.13$ | |
| 0.001 | 0.00000e+000 | 0.00000e+000 | 0.00000e+000 | 0.00000e+000 | 0.00000e+000 | 0.00000e+000 |
| 0.002 | 0.00000e+000 | 0.00000e+000 | 0.00000e+000 | 0.00000e+000 | 0.00000e+000 | 0.00000e+000 |
| 0.003 | 0.00000e+000 | 0.00000e+000 | 0.00000e+000 | 0.00000e+000 | 0.00000e+000 | 0.00000e+000 |
| 0.004 | 0.00000e+000 | 0.00000e+000 | 0.00000e+000 | 0.00000e+000 | 0.00000e+000 | 0.00000e+000 |
| 0.005 | 0.00000e+000 | 0.00000e+000 | 0.00000e+000 | 0.00000e+000 | 0.00000e+000 | 0.00000e+000 |
| 0.006 | 0.00000e+000 | 0.00000e+000 | 0.00000e+000 | 0.00000e+000 | 0.00000e+000 | 0.00000e+000 |
| 0.007 | 0.00000e+000 | 0.00000e+000 | 0.00000e+000 | 0.00000e+000 | 0.00000e+000 | 0.00000e+000 |
| 0.008 | 2.31501e−014 | 0.00000e+000 | 2.49719e−014 | 0.00000e+000 | 2.68628e−014 | 0.00000e+000 |
| 0.009 | 1.97797e−012 | 0.00000e+000 | 2.13376e−012 | 0.00000e+000 | 2.29546e−012 | 0.00000e+000 |
| 0.010 | 2.68231e−011 | 0.00000e+000 | 2.89375e−011 | 0.00000e+000 | 3.11322e−011 | 0.00000e+000 |
| 0.020 | 9.59548e−007 | 9.58967e−008 | 1.02192e−006 | 8.96235e−008 | 1.08718e−006 | 8.36133e−008 |
| 0.030 | 4.64277e−005 | 1.31792e−005 | 4.82271e−005 | 1.23138e−005 | 5.01663e−005 | 1.14852e−005 |
| 0.040 | 3.82004e−004 | 1.44440e−004 | 3.91699e−004 | 1.34915e−004 | 4.02555e−004 | 1.25800e−004 |
| 0.050 | 1.40726e−003 | 5.99497e−004 | 1.43351e−003 | 5.59751e−004 | 1.46409e−003 | 5.21744e−004 |
| 0.060 | 3.44667e−003 | 1.55725e−003 | 3.49867e−003 | 1.45333e−003 | 3.56147e−003 | 1.35403e−003 |
| 0.070 | 6.71030e−003 | 3.13314e−003 | 6.79777e−003 | 2.92245e−003 | 6.90672e−003 | 2.72127e−003 |
| 0.080 | 1.13327e−002 | 5.39814e−003 | 1.14663e−002 | 5.03202e−003 | 1.16369e−002 | 4.68268e−003 |
| 0.090 | 1.74055e−002 | 8.39629e−003 | 1.75969e−002 | 7.82155e−003 | 1.78465e−002 | 7.27358e−003 |
| 0.100 | 2.49939e−002 | 1.21565e−002 | 2.52564e−002 | 1.13164e−002 | 2.56043e−002 | 1.05161e−002 |
| 0.110 | 3.41372e−002 | 1.66942e−002 | 3.44852e−002 | 1.55294e−002 | 3.49526e−002 | 1.44207e−002 |
| 0.120 | 4.48437e−002 | 2.20100e−002 | 4.52928e−002 | 2.04599e−002 | 4.59022e−002 | 1.89855e−002 |
| 0.130 | 5.70870e−002 | 2.80882e−002 | 5.76533e−002 | 2.60923e−002 | 5.84282e−002 | 2.41955e−002 |
| 0.140 | 7.08066e−002 | 3.48974e−002 | 7.15070e−002 | 3.23969e−002 | 7.24712e−002 | 3.00223e−002 |
| 0.150 | 8.59108e−002 | 4.23916e−002 | 8.67619e−002 | 3.93306e−002 | 8.79392e−002 | 3.64260e−002 |
| 0.160 | 1.02281e−001 | 5.05131e−002 | 1.03300e−001 | 4.68402e−002 | 1.04713e−001 | 4.33576e−002 |
| 0.170 | 1.19778e−001 | 5.91955e−002 | 1.20980e−001 | 5.48645e−002 | 1.22652e−001 | 5.07610e−002 |
| 0.180 | 1.38246e−001 | 6.83649e−002 | 1.39645e−001 | 6.33360e−002 | 1.41596e−001 | 5.85750e−002 |
| 0.190 | 1.57516e−001 | 7.79427e−002 | 1.59124e−001 | 7.21830e−002 | 1.61372e−001 | 6.67340e−002 |
| 0.200 | 1.77414e−001 | 8.78491e−002 | 1.79243e−001 | 8.13332e−002 | 1.81804e−001 | 7.51730e−002 |
| 0.210 | 1.97771e−001 | 9.80058e−002 | 1.99829e−001 | 9.07157e−002 | 2.02714e−001 | 8.38280e−002 |
| 0.220 | 2.18425e−001 | 1.08340e−001 | 2.20719e−001 | 1.00264e−001 | 2.23938e−001 | 9.26391e−002 |
| 0.230 | 2.39238e−001 | 1.18785e−001 | 2.41774e−001 | 1.09920e−001 | 2.45332e−001 | 1.01554e−001 |
| 0.240 | 2.60089e−001 | 1.29289e−001 | 2.62869e−001 | 1.19634e−001 | 2.66770e−001 | 1.10528e−001 |
| 0.250 | 2.80890e−001 | 1.39805e−001 | 2.83914e−001 | 1.29366e−001 | 2.88160e−001 | 1.19524e−001 |
| 0.260 | 3.01568e−001 | 1.50301e−001 | 3.04838e−001 | 1.39085e−001 | 3.09428e−001 | 1.28516e−001 |
| 0.270 | 3.22077e−001 | 1.60752e−001 | 3.25590e−001 | 1.48769e−001 | 3.30522e−001 | 1.37483e−001 |
| 0.280 | 3.42377e−001 | 1.71138e−001 | 3.46133e−001 | 1.58400e−001 | 3.51406e−001 | 1.46407e−001 |
| 0.290 | 3.62450e−001 | 1.81444e−001 | 3.66444e−001 | 1.67963e−001 | 3.72053e−001 | 1.55276e−001 |
| 0.300 | 3.82269e−001 | 1.91660e−001 | 3.86501e−001 | 1.77450e−001 | 3.92443e−001 | 1.64081e−001 |
| 0.310 | 4.01829e−001 | 2.01780e−001 | 4.06292e−001 | 1.86853e−001 | 4.12562e−001 | 1.72816e−001 |
| 0.320 | 4.21121e−001 | 2.11795e−001 | 4.25814e−001 | 1.96167e−001 | 4.32408e−001 | 1.81473e−001 |
| 0.330 | 4.40139e−001 | 2.21701e−001 | 4.45058e−001 | 2.05384e−001 | 4.51965e−001 | 1.90049e−001 |
| 0.340 | 4.58876e−001 | 2.31496e−001 | 4.64014e−001 | 2.14505e−001 | 4.71231e−001 | 1.98540e−001 |
| 0.350 | 4.77334e−001 | 2.41177e−001 | 4.82687e−001 | 2.23526e−001 | 4.90207e−001 | 2.06944e−001 |
| 0.360 | 4.95514e−001 | 2.50740e−001 | 5.01077e−001 | 2.32443e−001 | 5.08893e−001 | 2.15258e−001 |
| 0.370 | 5.13411e−001 | 2.60188e−001 | 5.19181e−001 | 2.41258e−001 | 5.27286e−001 | 2.23482e−001 |
| 0.380 | 5.31034e−001 | 2.69518e−001 | 5.37001e−001 | 2.49968e−001 | 5.45390e−001 | 2.31614e−001 |
| 0.390 | 5.48382e−001 | 2.78727e−001 | 5.54544e−001 | 2.58572e−001 | 5.63205e−001 | 2.39652e−001 |
| 0.400 | 5.65454e−001 | 2.87820e−001 | 5.71806e−001 | 2.67072e−001 | 5.80738e−001 | 2.47598e−001 |
| 0.410 | 5.82263e−001 | 2.96797e−001 | 5.88799e−001 | 2.75469e−001 | 5.97990e−001 | 2.55454e−001 |
| 0.420 | 5.98803e−001 | 3.05652e−001 | 6.05516e−001 | 2.83756e−001 | 6.14960e−001 | 2.63211e−001 |
| 0.430 | 6.15091e−001 | 3.14398e−001 | 6.21975e−001 | 2.91947e−001 | 6.31661e−001 | 2.70883e−001 |
| 0.440 | 6.31117e−001 | 3.23023e−001 | 6.38166e−001 | 3.00029e−001 | 6.48089e−001 | 2.78456e−001 |
| 0.450 | 6.46897e−001 | 3.31539e−001 | 6.54110e−001 | 3.08013e−001 | 6.64265e−001 | 2.85944e−001 |
| 0.460 | 6.62428e−001 | 3.39941e−001 | 6.69796e−001 | 3.15895e−001 | 6.80172e−001 | 2.93339e−001 |
| 0.470 | 6.77719e−001 | 3.48235e−001 | 6.85238e−001 | 3.23679e−001 | 6.95831e−001 | 3.00646e−001 |
| 0.480 | 6.92777e−001 | 3.56416e−001 | 7.00440e−001 | 3.31362e−001 | 7.11245e−001 | 3.07864e−001 |
| 0.490 | 7.07604e−001 | 3.64494e−001 | 7.15404e−001 | 3.38952e−001 | 7.26412e−001 | 3.14997e−001 |
| 0.500 | 7.22206e−001 | 3.72463e−001 | 7.30147e−001 | 3.46444e−001 | 7.41348e−001 | 3.22042e−001 |
| 0.510 | 7.36587e−001 | 3.80330e−001 | 7.44658e−001 | 3.53843e−001 | 7.56049e−001 | 3.29002e−001 |
| 0.520 | 7.50756e−001 | 3.88094e−001 | 7.58952e−001 | 3.61148e−001 | 7.70526e−001 | 3.35879e−001 |
| 0.530 | 7.64715e−001 | 3.95757e−001 | 7.73033e−001 | 3.68364e−001 | 7.84784e−001 | 3.42673e−001 |
| 0.540 | 7.78470e−001 | 4.03324e−001 | 7.86906e−001 | 3.75490e−001 | 7.98826e−001 | 3.49387e−001 |
| 0.550 | 7.92025e−001 | 4.10792e−001 | 8.00572e−001 | 3.82528e−001 | 8.12660e−001 | 3.56020e−001 |
| 0.560 | 8.05388e−001 | 4.18165e−001 | 8.14043e−001 | 3.89479e−001 | 8.26290e−001 | 3.62575e−001 |
| 0.570 | 8.18556e−001 | 4.25446e−001 | 8.27315e−001 | 3.96346e−001 | 8.39717e−001 | 3.69053e−001 |
| 0.580 | 8.31543e−001 | 4.32635e−001 | 8.40401e−001 | 4.03129e−001 | 8.52955e−001 | 3.75454e−001 |
| 0.590 | 8.44349e−001 | 4.39734e−001 | 8.53302e−001 | 4.09830e−001 | 8.65999e−001 | 3.81780e−001 |
| 0.600 | 8.56978e−001 | 4.46747e−001 | 8.66025e−001 | 4.16452e−001 | 8.78860e−001 | 3.88035e−001 |
| 0.610 | 8.69437e−001 | 4.53671e−001 | 8.78572e−001 | 4.22992e−001 | 8.91541e−001 | 3.94215e−001 |
| 0.620 | 8.81726e−001 | 4.60512e−001 | 8.90947e−001 | 4.29457e−001 | 9.04046e−001 | 4.00325e−001 |
| 0.630 | 8.93854e−001 | 4.67268e−001 | 9.03155e−001 | 4.35844e−001 | 9.16378e−001 | 4.06364e−001 |
| 0.640 | 9.05822e−001 | 4.73945e−001 | 9.15203e−001 | 4.42158e−001 | 9.28545e−001 | 4.12336e−001 |
| 0.650 | 9.17635e−001 | 4.80539e−001 | 9.27091e−001 | 4.48396e−001 | 9.40548e−001 | 4.18237e−001 |
| 0.660 | 9.29291e−001 | 4.87056e−001 | 9.38818e−001 | 4.54563e−001 | 9.52387e−001 | 4.24074e−001 |
| 0.670 | 9.40805e−001 | 4.93497e−001 | 9.50401e−001 | 4.60660e−001 | 9.64078e−001 | 4.29847e−001 |
| 0.680 | 9.52168e−001 | 4.99860e−001 | 9.61831e−001 | 4.66686e−001 | 9.75609e−001 | 4.35552e−001 |
| 0.690 | 9.63393e−001 | 5.06152e−001 | 9.73121e−001 | 4.72645e−001 | 9.87000e−001 | 4.41198e−001 |
| 0.700 | 9.74475e−001 | 5.12367e−001 | 9.84263e−001 | 4.78534e−001 | 9.98239e−001 | 4.46778e−001 |

| | | | | | | |
|---|---|---|---|---|---|---|
| 0.710 | 9.85427e−001 | 5.18514e−001 | 9.95275e−001 | 4.84359e−001 | 1.00934e+000 | 4.52298e−001 |
| 0.720 | 9.96239e−001 | 5.24589e−001 | 1.00614e+000 | 4.90118e−001 | 1.02030e+000 | 4.57759e−001 |
| 0.730 | 1.00693e+000 | 5.30595e−001 | 1.01689e+000 | 4.95814e−001 | 1.03113e+000 | 4.63159e−001 |
| 0.740 | 1.01749e+000 | 5.36531e−001 | 1.02750e+000 | 5.01444e−001 | 1.04182e+000 | 4.68499e−001 |
| 0.750 | 1.02792e+000 | 5.42404e−001 | 1.03798e+000 | 5.07016e−001 | 1.05239e+000 | 4.73786e−001 |
| 0.760 | 1.03824e+000 | 5.48211e−001 | 1.04834e+000 | 5.12526e−001 | 1.06283e+000 | 4.79014e−001 |
| 0.770 | 1.04843e+000 | 5.53952e−001 | 1.05858e+000 | 5.17976e−001 | 1.07314e+000 | 4.84187e−001 |
| 0.780 | 1.05850e+000 | 5.59630e−001 | 1.06870e+000 | 5.23366e−001 | 1.08333e+000 | 4.89303e−001 |
| 0.790 | 1.06847e+000 | 5.65248e−001 | 1.07871e+000 | 5.28701e−001 | 1.09341e+000 | 4.94370e−001 |
| 0.800 | 1.07832e+000 | 5.70803e−001 | 1.08860e+000 | 5.33977e−001 | 1.10336e+000 | 4.99380e−001 |
| 0.810 | 1.08806e+000 | 5.76299e−001 | 1.09838e+000 | 5.39198e−001 | 1.11321e+000 | 5.04339e−001 |
| 0.820 | 1.09770e+000 | 5.81734e−001 | 1.10805e+000 | 5.44362e−001 | 1.12294e+000 | 5.09245e−001 |
| 0.830 | 1.10722e+000 | 5.87112e−001 | 1.11761e+000 | 5.49473e−001 | 1.13256e+000 | 5.14103e−001 |
| 0.840 | 1.11665e+000 | 5.92434e−001 | 1.12707e+000 | 5.54532e−001 | 1.14207e+000 | 5.18910e−001 |
| 0.850 | 1.12597e+000 | 5.97699e−001 | 1.13642e+000 | 5.59538e−001 | 1.15148e+000 | 5.23668e−001 |
| 0.860 | 1.13519e+000 | 6.02909e−001 | 1.14568e+000 | 5.64492e−001 | 1.16079e+000 | 5.28379e−001 |
| 0.870 | 1.14431e+000 | 6.08066e−001 | 1.15482e+000 | 5.69396e−001 | 1.16999e+000 | 5.33041e−001 |
| 0.880 | 1.15333e+000 | 6.13166e−001 | 1.16387e+000 | 5.74247e−001 | 1.17909e+000 | 5.37654e−001 |
| 0.890 | 1.16227e+000 | 6.18217e−001 | 1.17284e+000 | 5.79052e−001 | 1.18810e+000 | 5.42224e−001 |
| 0.900 | 1.17111e+000 | 6.23216e−001 | 1.18170e+000 | 5.83809e−001 | 1.19702e+000 | 5.46749e−001 |
| 0.910 | 1.17986e+000 | 6.28161e−001 | 1.19048e+000 | 5.88515e−001 | 1.20583e+000 | 5.51226e−001 |
| 0.920 | 1.18851e+000 | 6.33056e−001 | 1.19915e+000 | 5.93174e−001 | 1.21455e+000 | 5.55659e−001 |
| 0.930 | 1.19708e+000 | 6.37902e−001 | 1.20775e+000 | 5.97787e−001 | 1.22319e+000 | 5.60049e−001 |
| 0.940 | 1.20557e+000 | 6.42701e−001 | 1.21625e+000 | 6.02356e−001 | 1.23173e+000 | 5.64396e−001 |
| 0.950 | 1.21397e+000 | 6.47453e−001 | 1.22467e+000 | 6.06880e−001 | 1.24019e+000 | 5.68703e−001 |
| 0.960 | 1.22228e+000 | 6.52157e−001 | 1.23300e+000 | 6.11359e−001 | 1.24856e+000 | 5.72967e−001 |
| 0.970 | 1.23051e+000 | 6.56814e−001 | 1.24125e+000 | 6.15794e−001 | 1.25684e+000 | 5.77190e−001 |
| 0.980 | 1.23866e+000 | 6.61422e−001 | 1.24941e+000 | 6.20184e−001 | 1.26504e+000 | 5.81370e−001 |
| 0.990 | 1.24673e+000 | 6.65988e−001 | 1.25750e+000 | 6.24533e−001 | 1.27317e+000 | 5.85510e−001 |
| 1.000 | 1.25472e+000 | 6.70509e−001 | 1.26551e+000 | 6.28841e−001 | 1.28120e+000 | 5.89613e−001 |
| 1.010 | 1.26264e+000 | 6.74990e−001 | 1.27344e+000 | 6.33110e−001 | 1.28916e+000 | 5.93678e−001 |
| 1.020 | 1.27047e+000 | 6.79424e−001 | 1.28129e+000 | 6.37334e−001 | 1.29705e+000 | 5.97702e−001 |
| 1.030 | 1.27823e+000 | 6.83814e−001 | 1.28906e+000 | 6.41519e−001 | 1.30484e+000 | 6.01688e−001 |
| 1.040 | 1.28592e+000 | 6.88161e−001 | 1.29676e+000 | 6.45661e−001 | 1.31257e+000 | 6.05635e−001 |
| 1.050 | 1.29353e+000 | 6.92472e−001 | 1.30439e+000 | 6.49770e−001 | 1.32022e+000 | 6.09550e−001 |
| 1.060 | 1.30107e+000 | 6.96746e−001 | 1.31194e+000 | 6.53844e−001 | 1.32780e+000 | 6.13430e−001 |
| 1.070 | 1.30855e+000 | 7.00972e−001 | 1.31942e+000 | 6.57873e−001 | 1.33531e+000 | 6.17270e−001 |
| 1.080 | 1.31596e+000 | 7.05159e−001 | 1.32684e+000 | 6.61865e−001 | 1.34275e+000 | 6.21073e−001 |
| 1.090 | 1.32329e+000 | 7.09306e−001 | 1.33418e+000 | 6.65820e−001 | 1.35011e+000 | 6.24843e−001 |
| 1.100 | 1.33055e+000 | 7.13418e−001 | 1.34145e+000 | 6.69741e−001 | 1.35741e+000 | 6.28579e−001 |
| 1.110 | 1.33775e+000 | 7.17489e−001 | 1.34866e+000 | 6.73623e−001 | 1.36464e+000 | 6.32279e−001 |
| 1.120 | 1.34488e+000 | 7.21527e−001 | 1.35580e+000 | 6.77473e−001 | 1.37180e+000 | 6.35949e−001 |
| 1.130 | 1.35195e+000 | 7.25523e−001 | 1.36288e+000 | 6.81286e−001 | 1.37890e+000 | 6.39584e−001 |
| 1.140 | 1.35896e+000 | 7.29488e−001 | 1.36989e+000 | 6.85067e−001 | 1.38593e+000 | 6.43187e−001 |
| 1.150 | 1.36590e+000 | 7.33414e−001 | 1.37683e+000 | 6.88812e−001 | 1.39289e+000 | 6.46758e−001 |
| 1.160 | 1.37278e+000 | 7.37302e−001 | 1.38372e+000 | 6.92522e−001 | 1.39979e+000 | 6.50295e−001 |
| 1.170 | 1.37959e+000 | 7.41159e−001 | 1.39054e+000 | 6.96200e−001 | 1.40663e+000 | 6.53802e−001 |
| 1.180 | 1.38635e+000 | 7.44982e−001 | 1.39730e+000 | 6.99848e−001 | 1.41341e+000 | 6.57281e−001 |
| 1.190 | 1.39305e+000 | 7.48766e−001 | 1.40400e+000 | 7.03458e−001 | 1.42012e+000 | 6.60722e−001 |
| 1.200 | 1.39968e+000 | 7.52522e−001 | 1.41064e+000 | 7.07044e−001 | 1.42678e+000 | 6.64142e−001 |
| 1.210 | 1.40626e+000 | 7.56240e−001 | 1.41723e+000 | 7.10590e−001 | 1.43338e+000 | 6.67524e−001 |
| 1.220 | 1.41278e+000 | 7.59926e−001 | 1.42375e+000 | 7.14108e−001 | 1.43991e+000 | 6.70879e−001 |
| 1.230 | 1.41925e+000 | 7.63580e−001 | 1.43022e+000 | 7.17595e−001 | 1.44640e+000 | 6.74204e−001 |
| 1.240 | 1.42566e+000 | 7.67208e−001 | 1.43663e+000 | 7.21057e−001 | 1.45283e+000 | 6.77505e−001 |
| 1.250 | 1.43202e+000 | 7.70797e−001 | 1.44299e+000 | 7.24482e−001 | 1.45919e+000 | 6.80773e−001 |
| 1.260 | 1.43831e+000 | 7.74357e−001 | 1.44929e+000 | 7.27881e−001 | 1.46550e+000 | 6.84014e−001 |
| 1.270 | 1.44456e+000 | 7.77888e−001 | 1.45554e+000 | 7.31251e−001 | 1.47177e+000 | 6.87230e−001 |
| 1.280 | 1.45075e+000 | 7.81387e−001 | 1.46173e+000 | 7.34592e−001 | 1.47797e+000 | 6.90415e−001 |
| 1.290 | 1.45689e+000 | 7.84855e−001 | 1.46787e+000 | 7.37902e−001 | 1.48412e+000 | 6.93573e−001 |
| 1.300 | 1.46298e+000 | 7.88297e−001 | 1.47396e+000 | 7.41187e−001 | 1.49022e+000 | 6.96707e−001 |
| 1.310 | 1.46902e+000 | 7.91708e−001 | 1.48000e+000 | 7.44445e−001 | 1.49627e+000 | 6.99816e−001 |
| 1.320 | 1.47501e+000 | 7.95089e−001 | 1.48598e+000 | 7.47671e−001 | 1.50226e+000 | 7.02893e−001 |
| 1.330 | 1.48094e+000 | 7.98442e−001 | 1.49191e+000 | 7.50874e−001 | 1.50820e+000 | 7.05947e−001 |
| 1.340 | 1.48683e+000 | 8.01770e−001 | 1.49781e+000 | 7.54052e−001 | 1.51410e+000 | 7.08981e−001 |
| 1.350 | 1.49267e+000 | 8.05066e−001 | 1.50365e+000 | 7.57197e−001 | 1.51995e+000 | 7.11980e−001 |
| 1.360 | 1.49846e+000 | 8.08335e−001 | 1.50943e+000 | 7.60319e−001 | 1.52574e+000 | 7.14958e−001 |
| 1.370 | 1.50420e+000 | 8.11578e−001 | 1.51517e+000 | 7.63415e−001 | 1.53149e+000 | 7.17913e−001 |
| 1.380 | 1.50990e+000 | 8.14792e−001 | 1.52087e+000 | 7.66485e−001 | 1.53719e+000 | 7.20843e−001 |
| 1.390 | 1.51555e+000 | 8.17985e−001 | 1.52652e+000 | 7.69534e−001 | 1.54285e+000 | 7.23753e−001 |
| 1.400 | 1.52115e+000 | 8.21149e−001 | 1.53212e+000 | 7.72556e−001 | 1.54846e+000 | 7.26634e−001 |
| 1.410 | 1.52671e+000 | 8.24286e−001 | 1.53768e+000 | 7.75551e−001 | 1.55403e+000 | 7.29493e−001 |
| 1.420 | 1.53223e+000 | 8.27399e−001 | 1.54319e+000 | 7.78523e−001 | 1.55954e+000 | 7.32329e−001 |
| 1.430 | 1.53769e+000 | 8.30487e−001 | 1.54865e+000 | 7.81471e−001 | 1.56501e+000 | 7.35142e−001 |
| 1.440 | 1.54312e+000 | 8.33548e−001 | 1.55408e+000 | 7.84397e−001 | 1.57044e+000 | 7.37934e−001 |
| 1.450 | 1.54850e+000 | 8.36584e−001 | 1.55946e+000 | 7.87295e−001 | 1.57582e+000 | 7.40700e−001 |
| 1.460 | 1.55384e+000 | 8.39599e−001 | 1.56480e+000 | 7.90175e−001 | 1.58116e+000 | 7.43448e−001 |
| 1.470 | 1.55913e+000 | 8.42586e−001 | 1.57008e+000 | 7.93027e−001 | 1.58646e+000 | 7.46168e−001 |
| 1.480 | 1.56439e+000 | 8.45552e−001 | 1.57534e+000 | 7.95861e−001 | 1.59171e+000 | 7.48874e−001 |
| 1.490 | 1.56960e+000 | 8.48491e−001 | 1.58055e+000 | 7.98669e−001 | 1.59693e+000 | 7.51554e−001 |
| 1.500 | 1.57478e+000 | 8.51414e−001 | 1.58572e+000 | 8.01460e−001 | 1.60210e+000 | 7.54218e−001 |
| 1.510 | 1.57991e+000 | 8.54311e−001 | 1.59085e+000 | 8.04227e−001 | 1.60724e+000 | 7.56858e−001 |
| 1.520 | 1.58500e+000 | 8.57182e−001 | 1.59594e+000 | 8.06968e−001 | 1.61233e+000 | 7.59475e−001 |
| 1.530 | 1.59006e+000 | 8.60031e−001 | 1.60099e+000 | 8.09689e−001 | 1.61738e+000 | 7.62072e−001 |

| | | | | | | |
|---|---|---|---|---|---|---|
| 1.540 | 1.59507e+000 | 8.62859e−001 | 1.60600e+000 | 8.12393e−001 | 1.62239e+000 | 7.64651e−001 |
| 1.550 | 1.60005e+000 | 8.65661e−001 | 1.61097e+000 | 8.15069e−001 | 1.62737e+000 | 7.67206e−001 |
| 1.560 | 1.60499e+000 | 8.68451e−001 | 1.61590e+000 | 8.17734e−001 | 1.63231e+000 | 7.69747e−001 |
| 1.570 | 1.60989e+000 | 8.71217e−001 | 1.62080e+000 | 8.20375e−001 | 1.63720e+000 | 7.72269e−001 |
| 1.580 | 1.61475e+000 | 8.73957e−001 | 1.62566e+000 | 8.22994e−001 | 1.64206e+000 | 7.74769e−001 |
| 1.590 | 1.61958e+000 | 8.76681e−001 | 1.63048e+000 | 8.25596e−001 | 1.64689e+000 | 7.77252e−001 |
| 1.600 | 1.62437e+000 | 8.79374e−001 | 1.63526e+000 | 8.28170e−001 | 1.65168e+000 | 7.79708e−001 |
| 1.610 | 1.62911e+000 | 8.82053e−001 | 1.64001e+000 | 8.30728e−001 | 1.65642e+000 | 7.82151e−001 |
| 1.620 | 1.63383e+000 | 8.84712e−001 | 1.64472e+000 | 8.33268e−001 | 1.66114e+000 | 7.84575e−001 |
| 1.630 | 1.63852e+000 | 8.87353e−001 | 1.64940e+000 | 8.35791e−001 | 1.66582e+000 | 7.86986e−001 |
| 1.640 | 1.64316e+000 | 8.89971e−001 | 1.65404e+000 | 8.38293e−001 | 1.67046e+000 | 7.89369e−001 |
| 1.650 | 1.64778e+000 | 8.92570e−001 | 1.65865e+000 | 8.40776e−001 | 1.67507e+000 | 7.91740e−001 |
| 1.660 | 1.65235e+000 | 8.95150e−001 | 1.66323e+000 | 8.43240e−001 | 1.67965e+000 | 7.94094e−001 |
| 1.670 | 1.65690e+000 | 8.97713e−001 | 1.66776e+000 | 8.45690e−001 | 1.68418e+000 | 7.96430e−001 |
| 1.680 | 1.66141e+000 | 9.00256e−001 | 1.67227e+000 | 8.48120e−001 | 1.68868e+000 | 7.98750e−001 |
| 1.690 | 1.66589e+000 | 9.02780e−001 | 1.67674e+000 | 8.50530e−001 | 1.69316e+000 | 8.01052e−001 |
| 1.700 | 1.67034e+000 | 9.05286e−001 | 1.68119e+000 | 8.52924e−001 | 1.69761e+000 | 8.03335e−001 |
| 1.710 | 1.67476e+000 | 9.07769e−001 | 1.68560e+000 | 8.55298e−001 | 1.70202e+000 | 8.05602e−001 |
| 1.720 | 1.67914e+000 | 9.10238e−001 | 1.68997e+000 | 8.57657e−001 | 1.70640e+000 | 8.07854e−001 |
| 1.730 | 1.68348e+000 | 9.12687e−001 | 1.69432e+000 | 8.59996e−001 | 1.71074e+000 | 8.10088e−001 |
| 1.740 | 1.68780e+000 | 9.15121e−001 | 1.69863e+000 | 8.62320e−001 | 1.71505e+000 | 8.12305e−001 |
| 1.750 | 1.69209e+000 | 9.17536e−001 | 1.70291e+000 | 8.64629e−001 | 1.71933e+000 | 8.14509e−001 |
| 1.760 | 1.69634e+000 | 9.19935e−001 | 1.70716e+000 | 8.66922e−001 | 1.72358e+000 | 8.16697e−001 |
| 1.770 | 1.70057e+000 | 9.22309e−001 | 1.71138e+000 | 8.69191e−001 | 1.72780e+000 | 8.18863e−001 |
| 1.780 | 1.70476e+000 | 9.24670e−001 | 1.71557e+000 | 8.71445e−001 | 1.73199e+000 | 8.21015e−001 |
| 1.790 | 1.70893e+000 | 9.27013e−001 | 1.71973e+000 | 8.73684e−001 | 1.73615e+000 | 8.23152e−001 |
| 1.800 | 1.71306e+000 | 9.29345e−001 | 1.72386e+000 | 8.75913e−001 | 1.74027e+000 | 8.25281e−001 |
| 1.810 | 1.71717e+000 | 9.31664e−001 | 1.72796e+000 | 8.78128e−001 | 1.74437e+000 | 8.27394e−001 |
| 1.820 | 1.72125e+000 | 9.33958e−001 | 1.73203e+000 | 8.80319e−001 | 1.74845e+000 | 8.29484e−001 |
| 1.830 | 1.72530e+000 | 9.36236e−001 | 1.73608e+000 | 8.82496e−001 | 1.75249e+000 | 8.31564e−001 |
| 1.840 | 1.72932e+000 | 9.38501e−001 | 1.74010e+000 | 8.84662e−001 | 1.75651e+000 | 8.33630e−001 |
| 1.850 | 1.73332e+000 | 9.40751e−001 | 1.74409e+000 | 8.86811e−001 | 1.76050e+000 | 8.35683e−001 |
| 1.860 | 1.73729e+000 | 9.42984e−001 | 1.74805e+000 | 8.88943e−001 | 1.76446e+000 | 8.37717e−001 |
| 1.870 | 1.74123e+000 | 9.45202e−001 | 1.75198e+000 | 8.91064e−001 | 1.76839e+000 | 8.39742e−001 |
| 1.880 | 1.74514e+000 | 9.47402e−001 | 1.75589e+000 | 8.93166e−001 | 1.77229e+000 | 8.41749e−001 |
| 1.890 | 1.74901e+000 | 9.49588e−001 | 1.75976e+000 | 8.95256e−001 | 1.77617e+000 | 8.43744e−001 |
| 1.900 | 1.75287e+000 | 9.51756e−001 | 1.76361e+000 | 8.97327e−001 | 1.78002e+000 | 8.45720e−001 |
| 1.910 | 1.75670e+000 | 9.53909e−001 | 1.76744e+000 | 8.99385e−001 | 1.78384e+000 | 8.47684e−001 |
| 1.920 | 1.76050e+000 | 9.56050e−001 | 1.77123e+000 | 9.01430e−001 | 1.78764e+000 | 8.49636e−001 |
| 1.930 | 1.76428e+000 | 9.58175e−001 | 1.77501e+000 | 9.03460e−001 | 1.79141e+000 | 8.51575e−001 |
| 1.940 | 1.76804e+000 | 9.60292e−001 | 1.77875e+000 | 9.05484e−001 | 1.79515e+000 | 8.53506e−001 |
| 1.950 | 1.77176e+000 | 9.62392e−001 | 1.78247e+000 | 9.07489e−001 | 1.79887e+000 | 8.55420e−001 |
| 1.960 | 1.77548e+000 | 9.64474e−001 | 1.78618e+000 | 9.09479e−001 | 1.80258e+000 | 8.57320e−001 |
| 1.970 | 1.77916e+000 | 9.66547e−001 | 1.78985e+000 | 9.11461e−001 | 1.80625e+000 | 8.59211e−001 |
| 1.980 | 1.78282e+000 | 9.68605e−001 | 1.79350e+000 | 9.13427e−001 | 1.80989e+000 | 8.61087e−001 |
| 1.990 | 1.78644e+000 | 9.70644e−001 | 1.79712e+000 | 9.15374e−001 | 1.81351e+000 | 8.62947e−001 |
| 2.000 | 1.79004e+000 | 9.72673e−001 | 1.80072e+000 | 9.17316e−001 | 1.81710e+000 | 8.64800e−001 |
| 2.010 | 1.79363e+000 | 9.74687e−001 | 1.80430e+000 | 9.19237e−001 | 1.82069e+000 | 8.66634e−001 |
| 2.020 | 1.79718e+000 | 9.76685e−001 | 1.80785e+000 | 9.21146e−001 | 1.82423e+000 | 8.68457e−001 |
| 2.030 | 1.80072e+000 | 9.78673e−001 | 1.81138e+000 | 9.23048e−001 | 1.82776e+000 | 8.70271e−001 |
| 2.040 | 1.80423e+000 | 9.80650e−001 | 1.81488e+000 | 9.24937e−001 | 1.83126e+000 | 8.72074e−001 |
| 2.050 | 1.80771e+000 | 9.82607e−001 | 1.81836e+000 | 9.26807e−001 | 1.83474e+000 | 8.73860e−001 |
| 2.060 | 1.81118e+000 | 9.84555e−001 | 1.82182e+000 | 9.28668e−001 | 1.83819e+000 | 8.75636e−001 |
| 2.070 | 1.81463e+000 | 9.86493e−001 | 1.82526e+000 | 9.30520e−001 | 1.84163e+000 | 8.77404e−001 |
| 2.080 | 1.81805e+000 | 9.88418e−001 | 1.82868e+000 | 9.32359e−001 | 1.84504e+000 | 8.79159e−001 |
| 2.090 | 1.82144e+000 | 9.90331e−001 | 1.83206e+000 | 9.34187e−001 | 1.84843e+000 | 8.80904e−001 |
| 2.100 | 1.82481e+000 | 9.92224e−001 | 1.83543e+000 | 9.35998e−001 | 1.85179e+000 | 8.82634e−001 |
| 2.110 | 1.82817e+000 | 9.94118e−001 | 1.83878e+000 | 9.37805e−001 | 1.85514e+000 | 8.84358e−001 |
| 2.120 | 1.83150e+000 | 9.95994e−001 | 1.84211e+000 | 9.39601e−001 | 1.85847e+000 | 8.86070e−001 |
| 2.130 | 1.83483e+000 | 9.97854e−001 | 1.84542e+000 | 9.41377e−001 | 1.86178e+000 | 8.87766e−001 |
| 2.140 | 1.83811e+000 | 9.99701e−001 | 1.84870e+000 | 9.43141e−001 | 1.86505e+000 | 8.89451e−001 |
| 2.150 | 1.84138e+000 | 1.00154e+000 | 1.85197e+000 | 9.44895e−001 | 1.86831e+000 | 8.91125e−001 |
| 2.160 | 1.84463e+000 | 1.00336e+000 | 1.85521e+000 | 9.46641e−001 | 1.87156e+000 | 8.92791e−001 |
| 2.170 | 1.84785e+000 | 1.00518e+000 | 1.85843e+000 | 9.48375e−001 | 1.87477e+000 | 8.94447e−001 |
| 2.180 | 1.85106e+000 | 1.00699e+000 | 1.86164e+000 | 9.50103e−001 | 1.87798e+000 | 8.96097e−001 |
| 2.190 | 1.85425e+000 | 1.00878e+000 | 1.86482e+000 | 9.51814e−001 | 1.88116e+000 | 8.97728e−001 |
| 2.200 | 1.85742e+000 | 1.01056e+000 | 1.86797e+000 | 9.53517e−001 | 1.88432e+000 | 8.99355e−001 |
| 2.210 | 1.86056e+000 | 1.01233e+000 | 1.87111e+000 | 9.55206e−001 | 1.88746e+000 | 9.00967e−001 |
| 2.220 | 1.86369e+000 | 1.01408e+000 | 1.87424e+000 | 9.56882e−001 | 1.89058e+000 | 9.02567e−001 |
| 2.230 | 1.86680e+000 | 1.01582e+000 | 1.87734e+000 | 9.58548e−001 | 1.89367e+000 | 9.04155e−001 |
| 2.240 | 1.86990e+000 | 1.01756e+000 | 1.88043e+000 | 9.60210e−001 | 1.89676e+000 | 9.05744e−001 |
| 2.250 | 1.87297e+000 | 1.01929e+000 | 1.88349e+000 | 9.61861e−001 | 1.89981e+000 | 9.07319e−001 |
| 2.260 | 1.87601e+000 | 1.02101e+000 | 1.88653e+000 | 9.63499e−001 | 1.90285e+000 | 9.08882e−001 |
| 2.270 | 1.87904e+000 | 1.02271e+000 | 1.88956e+000 | 9.65130e−001 | 1.90588e+000 | 9.10439e−001 |
| 2.280 | 1.88207e+000 | 1.02441e+000 | 1.89257e+000 | 9.66752e−001 | 1.90889e+000 | 9.11987e−001 |
| 2.290 | 1.88506e+000 | 1.02610e+000 | 1.89556e+000 | 9.68362e−001 | 1.91188e+000 | 9.13526e−001 |
| 2.300 | 1.88804e+000 | 1.02777e+000 | 1.89854e+000 | 9.69960e−001 | 1.91485e+000 | 9.15048e−001 |
| 2.310 | 1.89100e+000 | 1.02943e+000 | 1.90149e+000 | 9.71547e−001 | 1.91780e+000 | 9.16564e−001 |
| 2.320 | 1.89394e+000 | 1.03108e+000 | 1.90442e+000 | 9.73122e−001 | 1.92073e+000 | 9.18069e−001 |
| 2.330 | 1.89685e+000 | 1.03272e+000 | 1.90733e+000 | 9.74693e−001 | 1.92363e+000 | 9.19566e−001 |
| 2.340 | 1.89976e+000 | 1.03435e+000 | 1.91023e+000 | 9.76251e−001 | 1.92653e+000 | 9.21052e−001 |
| 2.350 | 1.90264e+000 | 1.03597e+000 | 1.91311e+000 | 9.77797e−001 | 1.92941e+000 | 9.22529e−001 |
| 2.360 | 1.90552e+000 | 1.03759e+000 | 1.91598e+000 | 9.79343e−001 | 1.93227e+000 | 9.24004e−001 |

| | | | | | | |
|---|---|---|---|---|---|---|
| 2.370 | 1.90837e+000 | 1.03919e+000 | 1.91883e+000 | 9.80875e−001 | 1.93511e+000 | 9.25466e−001 |
| 2.380 | 1.91121e+000 | 1.04078e+000 | 1.92165e+000 | 9.82392e−001 | 1.93794e+000 | 9.26914e−001 |
| 2.390 | 1.91402e+000 | 1.04236e+000 | 1.92447e+000 | 9.83903e−001 | 1.94075e+000 | 9.28355e−001 |
| 2.400 | 1.91683e+000 | 1.04394e+000 | 1.92727e+000 | 9.85411e−001 | 1.94355e+000 | 9.29796e−001 |
| 2.410 | 1.91962e+000 | 1.04550e+000 | 1.93006e+000 | 9.86907e−001 | 1.94633e+000 | 9.31224e−001 |
| 2.420 | 1.92240e+000 | 1.04706e+000 | 1.93282e+000 | 9.88394e−001 | 1.94909e+000 | 9.32644e−001 |
| 2.430 | 1.92515e+000 | 1.04861e+000 | 1.93557e+000 | 9.89880e−001 | 1.95184e+000 | 9.34060e−001 |
| 2.440 | 1.92789e+000 | 1.05015e+000 | 1.93830e+000 | 9.91351e−001 | 1.95457e+000 | 9.35465e−001 |
| 2.450 | 1.93062e+000 | 1.05168e+000 | 1.94102e+000 | 9.92811e−001 | 1.95729e+000 | 9.36858e−001 |
| 2.460 | 1.93333e+000 | 1.05320e+000 | 1.94372e+000 | 9.94263e−001 | 1.95999e+000 | 9.38246e−001 |
| 2.470 | 1.93601e+000 | 1.05472e+000 | 1.94641e+000 | 9.95711e−001 | 1.96267e+000 | 9.39627e−001 |
| 2.480 | 1.93869e+000 | 1.05622e+000 | 1.94908e+000 | 9.97145e−001 | 1.96534e+000 | 9.40994e−001 |
| 2.490 | 1.94135e+000 | 1.05771e+000 | 1.95173e+000 | 9.98575e−001 | 1.96799e+000 | 9.42360e−001 |
| 2.500 | 1.94399e+000 | 1.05920e+000 | 1.95437e+000 | 9.99991e−001 | 1.97062e+000 | 9.43712e−001 |
| 2.550 | 1.95697e+000 | 1.06648e+000 | 1.96733e+000 | 1.00695e+000 | 1.98356e+000 | 9.50357e−001 |
| 2.600 | 1.96960e+000 | 1.07357e+000 | 1.97992e+000 | 1.01372e+000 | 1.99613e+000 | 9.56814e−001 |
| 2.650 | 1.98187e+000 | 1.08046e+000 | 1.99216e+000 | 1.02030e+000 | 2.00837e+000 | 9.63097e−001 |
| 2.700 | 1.99382e+000 | 1.08718e+000 | 2.00409e+000 | 1.02672e+000 | 2.02027e+000 | 9.69224e−001 |
| 2.750 | 2.00545e+000 | 1.09369e+000 | 2.01569e+000 | 1.03295e+000 | 2.03187e+000 | 9.75162e−001 |
| 2.800 | 2.01677e+000 | 1.10004e+000 | 2.02698e+000 | 1.03902e+000 | 2.04314e+000 | 9.80953e−001 |
| 2.850 | 2.02777e+000 | 1.10622e+000 | 2.03795e+000 | 1.04492e+000 | 2.05410e+000 | 9.86586e−001 |
| 2.900 | 2.03848e+000 | 1.11223e+000 | 2.04864e+000 | 1.05066e+000 | 2.06478e+000 | 9.92063e−001 |
| 2.950 | 2.04892e+000 | 1.11808e+000 | 2.05906e+000 | 1.05625e+000 | 2.07518e+000 | 9.97400e−001 |
| 3.000 | 2.05912e+000 | 1.12380e+000 | 2.06923e+000 | 1.06172e+000 | 2.08533e+000 | 1.00261e+000 |
| 3.050 | 2.06907e+000 | 1.12939e+000 | 2.07916e+000 | 1.06705e+000 | 2.09525e+000 | 1.00770e+000 |
| 3.100 | 2.07876e+000 | 1.13482e+000 | 2.08882e+000 | 1.07224e+000 | 2.10490e+000 | 1.01266e+000 |
| 3.150 | 2.08821e+000 | 1.14011e+000 | 2.09824e+000 | 1.07730e+000 | 2.11430e+000 | 1.01748e+000 |
| 3.200 | 2.09742e+000 | 1.14528e+000 | 2.10744e+000 | 1.08223e+000 | 2.12349e+000 | 1.02219e+000 |
| 3.250 | 2.10639e+000 | 1.15032e+000 | 2.11639e+000 | 1.08705e+000 | 2.13241e+000 | 1.02678e+000 |
| 3.300 | 2.11517e+000 | 1.15523e+000 | 2.12515e+000 | 1.09174e+000 | 2.14116e+000 | 1.03126e+000 |
| 3.350 | 2.12375e+000 | 1.16005e+000 | 2.13371e+000 | 1.09634e+000 | 2.14970e+000 | 1.03565e+000 |
| 3.400 | 2.13216e+000 | 1.16475e+000 | 2.14209e+000 | 1.10084e+000 | 2.15808e+000 | 1.03994e+000 |
| 3.450 | 2.14035e+000 | 1.16935e+000 | 2.15026e+000 | 1.10523e+000 | 2.16624e+000 | 1.04413e+000 |
| 3.500 | 2.14837e+000 | 1.17384e+000 | 2.15825e+000 | 1.10952e+000 | 2.17422e+000 | 1.04822e+000 |
| 3.550 | 2.15618e+000 | 1.17822e+000 | 2.16605e+000 | 1.11370e+000 | 2.18201e+000 | 1.05221e+000 |
| 3.600 | 2.16382e+000 | 1.18251e+000 | 2.17367e+000 | 1.11779e+000 | 2.18961e+000 | 1.05612e+000 |
| 3.650 | 2.17131e+000 | 1.18670e+000 | 2.18113e+000 | 1.12180e+000 | 2.19706e+000 | 1.05994e+000 |
| 3.700 | 2.17861e+000 | 1.19079e+000 | 2.18842e+000 | 1.12571e+000 | 2.20434e+000 | 1.06367e+000 |
| 3.750 | 2.18576e+000 | 1.19479e+000 | 2.19556e+000 | 1.12952e+000 | 2.21146e+000 | 1.06731e+000 |
| 3.800 | 2.19279e+000 | 1.19873e+000 | 2.20255e+000 | 1.13329e+000 | 2.21845e+000 | 1.07090e+000 |
| 3.850 | 2.19967e+000 | 1.20259e+000 | 2.20942e+000 | 1.13698e+000 | 2.22530e+000 | 1.07442e+000 |
| 3.900 | 2.20641e+000 | 1.20636e+000 | 2.21615e+000 | 1.14058e+000 | 2.23201e+000 | 1.07785e+000 |
| 3.950 | 2.21299e+000 | 1.21005e+000 | 2.22271e+000 | 1.14409e+000 | 2.23857e+000 | 1.08121e+000 |
| 4.000 | 2.21942e+000 | 1.21365e+000 | 2.22912e+000 | 1.14754e+000 | 2.24497e+000 | 1.08449e+000 |
| 4.050 | 2.22573e+000 | 1.21718e+000 | 2.23542e+000 | 1.15092e+000 | 2.25125e+000 | 1.08771e+000 |
| 4.100 | 2.23193e+000 | 1.22065e+000 | 2.24159e+000 | 1.15422e+000 | 2.25742e+000 | 1.09086e+000 |
| 4.150 | 2.23797e+000 | 1.22404e+000 | 2.24762e+000 | 1.15746e+000 | 2.26344e+000 | 1.09395e+000 |
| 4.200 | 2.24391e+000 | 1.22737e+000 | 2.25355e+000 | 1.16064e+000 | 2.26935e+000 | 1.09699e+000 |
| 4.250 | 2.24975e+000 | 1.23063e+000 | 2.25937e+000 | 1.16375e+000 | 2.27516e+000 | 1.09995e+000 |
| 4.300 | 2.25548e+000 | 1.23384e+000 | 2.26509e+000 | 1.16682e+000 | 2.28088e+000 | 1.10288e+000 |
| 4.350 | 2.26110e+000 | 1.23699e+000 | 2.27069e+000 | 1.16983e+000 | 2.28647e+000 | 1.10575e+000 |
| 4.400 | 2.26661e+000 | 1.24008e+000 | 2.27619e+000 | 1.17278e+000 | 2.29196e+000 | 1.10856e+000 |
| 4.450 | 2.27202e+000 | 1.24309e+000 | 2.28159e+000 | 1.17566e+000 | 2.29735e+000 | 1.11131e+000 |
| 4.500 | 2.27731e+000 | 1.24606e+000 | 2.28686e+000 | 1.17849e+000 | 2.30260e+000 | 1.11401e+000 |
| 4.550 | 2.28249e+000 | 1.24897e+000 | 2.29202e+000 | 1.18127e+000 | 2.30776e+000 | 1.11665e+000 |
| 4.600 | 2.28760e+000 | 1.25182e+000 | 2.29712e+000 | 1.18399e+000 | 2.31285e+000 | 1.11925e+000 |
| 4.650 | 2.29261e+000 | 1.25462e+000 | 2.30212e+000 | 1.18666e+000 | 2.31784e+000 | 1.12180e+000 |
| 4.700 | 2.29753e+000 | 1.25739e+000 | 2.30702e+000 | 1.18930e+000 | 2.32273e+000 | 1.12432e+000 |
| 4.750 | 2.30238e+000 | 1.26010e+000 | 2.31186e+000 | 1.19189e+000 | 2.32757e+000 | 1.12679e+000 |
| 4.800 | 2.30714e+000 | 1.26275e+000 | 2.31660e+000 | 1.19443e+000 | 2.33230e+000 | 1.12921e+000 |
| 4.850 | 2.31181e+000 | 1.26536e+000 | 2.32127e+000 | 1.19692e+000 | 2.33695e+000 | 1.13159e+000 |
| 4.900 | 2.31638e+000 | 1.26793e+000 | 2.32583e+000 | 1.19937e+000 | 2.34151e+000 | 1.13392e+000 |
| 4.950 | 2.32090e+000 | 1.27046e+000 | 2.33033e+000 | 1.20179e+000 | 2.34600e+000 | 1.13622e+000 |
| 5.000 | 2.32531e+000 | 1.27291e+000 | 2.33472e+000 | 1.20413e+000 | 2.35039e+000 | 1.13846e+000 |
| 5.050 | 2.32966e+000 | 1.27534e+000 | 2.33907e+000 | 1.20645e+000 | 2.35472e+000 | 1.14067e+000 |
| 5.100 | 2.33394e+000 | 1.27774e+000 | 2.34333e+000 | 1.20874e+000 | 2.35898e+000 | 1.14286e+000 |
| 5.150 | 2.33815e+000 | 1.28010e+000 | 2.34754e+000 | 1.21099e+000 | 2.36318e+000 | 1.14500e+000 |
| 5.200 | 2.34230e+000 | 1.28241e+000 | 2.35167e+000 | 1.21320e+000 | 2.36730e+000 | 1.14711e+000 |
| 5.250 | 2.34638e+000 | 1.28469e+000 | 2.35574e+000 | 1.21538e+000 | 2.37136e+000 | 1.14919e+000 |
| 5.300 | 2.35039e+000 | 1.28694e+000 | 2.35974e+000 | 1.21752e+000 | 2.37536e+000 | 1.15123e+000 |
| 5.350 | 2.35433e+000 | 1.28914e+000 | 2.36367e+000 | 1.21963e+000 | 2.37928e+000 | 1.15324e+000 |
| 5.400 | 2.35821e+000 | 1.29131e+000 | 2.36754e+000 | 1.22170e+000 | 2.38314e+000 | 1.15521e+000 |
| 5.450 | 2.36203e+000 | 1.29345e+000 | 2.37135e+000 | 1.22373e+000 | 2.38695e+000 | 1.15715e+000 |
| 5.500 | 2.36579e+000 | 1.29555e+000 | 2.37510e+000 | 1.22574e+000 | 2.39069e+000 | 1.15906e+000 |
| 5.550 | 2.36949e+000 | 1.29762e+000 | 2.37878e+000 | 1.22772e+000 | 2.39437e+000 | 1.16095e+000 |
| 5.600 | 2.37313e+000 | 1.29966e+000 | 2.38242e+000 | 1.22966e+000 | 2.39800e+000 | 1.16281e+000 |
| 5.650 | 2.37672e+000 | 1.30166e+000 | 2.38600e+000 | 1.23158e+000 | 2.40157e+000 | 1.16463e+000 |
| 5.700 | 2.38026e+000 | 1.30364e+000 | 2.38953e+000 | 1.23347e+000 | 2.40510e+000 | 1.16643e+000 |
| 5.750 | 2.38374e+000 | 1.30558e+000 | 2.39300e+000 | 1.23532e+000 | 2.40856e+000 | 1.16820e+000 |
| 5.800 | 2.38716e+000 | 1.30749e+000 | 2.39641e+000 | 1.23715e+000 | 2.41196e+000 | 1.16994e+000 |
| 5.850 | 2.39053e+000 | 1.30938e+000 | 2.39978e+000 | 1.23895e+000 | 2.41533e+000 | 1.17166e+000 |
| 5.900 | 2.39387e+000 | 1.31124e+000 | 2.40309e+000 | 1.24072e+000 | 2.41863e+000 | 1.17335e+000 |
| 5.950 | 2.39715e+000 | 1.31307e+000 | 2.40637e+000 | 1.24247e+000 | 2.42191e+000 | 1.17502e+000 |

| | | | | | | |
|---|---|---|---|---|---|---|
| 6.000 | 2.40038e+000 | 1.31488e+000 | 2.40959e+000 | 1.24420e+000 | 2.42512e+000 | 1.17667e+000 |
| 6.050 | 2.40356e+000 | 1.31666e+000 | 2.41276e+000 | 1.24590e+000 | 2.42828e+000 | 1.17828e+000 |
| 6.100 | 2.40669e+000 | 1.31841e+000 | 2.41589e+000 | 1.24757e+000 | 2.43141e+000 | 1.17988e+000 |
| 6.150 | 2.40979e+000 | 1.32014e+000 | 2.41898e+000 | 1.24921e+000 | 2.43449e+000 | 1.18145e+000 |
| 6.200 | 2.41284e+000 | 1.32184e+000 | 2.42201e+000 | 1.25084e+000 | 2.43752e+000 | 1.18300e+000 |
| 6.250 | 2.41584e+000 | 1.32352e+000 | 2.42501e+000 | 1.25244e+000 | 2.44052e+000 | 1.18452e+000 |
| 6.300 | 2.41880e+000 | 1.32518e+000 | 2.42796e+000 | 1.25403e+000 | 2.44346e+000 | 1.18603e+000 |
| 6.350 | 2.42172e+000 | 1.32681e+000 | 2.43088e+000 | 1.25559e+000 | 2.44637e+000 | 1.18752e+000 |
| 6.400 | 2.42461e+000 | 1.32842e+000 | 2.43375e+000 | 1.25712e+000 | 2.44924e+000 | 1.18898e+000 |
| 6.450 | 2.42745e+000 | 1.33001e+000 | 2.43659e+000 | 1.25864e+000 | 2.45207e+000 | 1.19043e+000 |
| 6.500 | 2.43025e+000 | 1.33158e+000 | 2.43939e+000 | 1.26013e+000 | 2.45486e+000 | 1.19186e+000 |
| 6.550 | 2.43302e+000 | 1.33312e+000 | 2.44215e+000 | 1.26161e+000 | 2.45762e+000 | 1.19326e+000 |
| 6.600 | 2.43575e+000 | 1.33464e+000 | 2.44486e+000 | 1.26306e+000 | 2.46033e+000 | 1.19464e+000 |
| 6.650 | 2.43844e+000 | 1.33614e+000 | 2.44755e+000 | 1.26449e+000 | 2.46301e+000 | 1.19601e+000 |
| 6.700 | 2.44110e+000 | 1.33763e+000 | 2.45020e+000 | 1.26591e+000 | 2.46565e+000 | 1.19736e+000 |
| 6.750 | 2.44372e+000 | 1.33910e+000 | 2.45281e+000 | 1.26731e+000 | 2.46826e+000 | 1.19870e+000 |
| 6.800 | 2.44631e+000 | 1.34054e+000 | 2.45539e+000 | 1.26869e+000 | 2.47084e+000 | 1.20001e+000 |
| 6.850 | 2.44886e+000 | 1.34196e+000 | 2.45794e+000 | 1.27005e+000 | 2.47339e+000 | 1.20131e+000 |
| 6.900 | 2.45137e+000 | 1.34337e+000 | 2.46044e+000 | 1.27139e+000 | 2.47588e+000 | 1.20259e+000 |
| 6.950 | 2.45385e+000 | 1.34475e+000 | 2.46292e+000 | 1.27271e+000 | 2.47836e+000 | 1.20385e+000 |
| 7.000 | 2.45631e+000 | 1.34613e+000 | 2.46537e+000 | 1.27402e+000 | 2.48080e+000 | 1.20510e+000 |
| 7.050 | 2.45874e+000 | 1.34748e+000 | 2.46779e+000 | 1.27531e+000 | 2.48322e+000 | 1.20632e+000 |
| 7.100 | 2.46113e+000 | 1.34881e+000 | 2.47018e+000 | 1.27659e+000 | 2.48560e+000 | 1.20754e+000 |
| 7.150 | 2.46350e+000 | 1.35014e+000 | 2.47254e+000 | 1.27785e+000 | 2.48796e+000 | 1.20875e+000 |
| 7.200 | 2.46584e+000 | 1.35145e+000 | 2.47487e+000 | 1.27910e+000 | 2.49029e+000 | 1.20993e+000 |
| 7.250 | 2.46815e+000 | 1.35274e+000 | 2.47717e+000 | 1.28033e+000 | 2.49258e+000 | 1.21111e+000 |
| 7.300 | 2.47043e+000 | 1.35401e+000 | 2.47944e+000 | 1.28155e+000 | 2.49485e+000 | 1.21227e+000 |
| 7.350 | 2.47267e+000 | 1.35527e+000 | 2.48169e+000 | 1.28275e+000 | 2.49709e+000 | 1.21341e+000 |
| 7.400 | 2.47489e+000 | 1.35650e+000 | 2.48390e+000 | 1.28392e+000 | 2.49930e+000 | 1.21453e+000 |
| 7.450 | 2.47709e+000 | 1.35772e+000 | 2.48609e+000 | 1.28509e+000 | 2.50149e+000 | 1.21564e+000 |
| 7.500 | 2.47925e+000 | 1.35893e+000 | 2.48825e+000 | 1.28624e+000 | 2.50364e+000 | 1.21674e+000 |
| 7.550 | 2.48139e+000 | 1.36012e+000 | 2.49038e+000 | 1.28738e+000 | 2.50576e+000 | 1.21783e+000 |
| 7.600 | 2.48351e+000 | 1.36130e+000 | 2.49249e+000 | 1.28851e+000 | 2.50787e+000 | 1.21890e+000 |
| 7.650 | 2.48559e+000 | 1.36247e+000 | 2.49456e+000 | 1.28962e+000 | 2.50995e+000 | 1.21996e+000 |
| 7.700 | 2.48765e+000 | 1.36362e+000 | 2.49663e+000 | 1.29072e+000 | 2.51201e+000 | 1.22101e+000 |
| 7.750 | 2.48970e+000 | 1.36477e+000 | 2.49867e+000 | 1.29181e+000 | 2.51404e+000 | 1.22205e+000 |
| 7.800 | 2.49173e+000 | 1.36590e+000 | 2.50069e+000 | 1.29289e+000 | 2.51606e+000 | 1.22308e+000 |
| 7.850 | 2.49373e+000 | 1.36702e+000 | 2.50268e+000 | 1.29396e+000 | 2.51805e+000 | 1.22410e+000 |
| 7.900 | 2.49571e+000 | 1.36811e+000 | 2.50466e+000 | 1.29501e+000 | 2.52002e+000 | 1.22510e+000 |
| 7.950 | 2.49766e+000 | 1.36921e+000 | 2.50661e+000 | 1.29605e+000 | 2.52197e+000 | 1.22609e+000 |
| 8.000 | 2.49960e+000 | 1.37028e+000 | 2.50854e+000 | 1.29708e+000 | 2.52389e+000 | 1.22707e+000 |
| 8.050 | 2.50151e+000 | 1.37135e+000 | 2.51045e+000 | 1.29810e+000 | 2.52580e+000 | 1.22804e+000 |
| 8.100 | 2.50339e+000 | 1.37240e+000 | 2.51232e+000 | 1.29910e+000 | 2.52767e+000 | 1.22900e+000 |
| 8.150 | 2.50526e+000 | 1.37345e+000 | 2.51418e+000 | 1.30009e+000 | 2.52952e+000 | 1.22995e+000 |
| 8.200 | 2.50710e+000 | 1.37448e+000 | 2.51602e+000 | 1.30108e+000 | 2.53136e+000 | 1.23088e+000 |
| 8.250 | 2.50892e+000 | 1.37549e+000 | 2.51783e+000 | 1.30205e+000 | 2.53317e+000 | 1.23181e+000 |
| 8.300 | 2.51072e+000 | 1.37649e+000 | 2.51963e+000 | 1.30300e+000 | 2.53496e+000 | 1.23271e+000 |
| 8.350 | 2.51249e+000 | 1.37748e+000 | 2.52140e+000 | 1.30395e+000 | 2.53673e+000 | 1.23362e+000 |
| 8.400 | 2.51426e+000 | 1.37846e+000 | 2.52316e+000 | 1.30489e+000 | 2.53848e+000 | 1.23451e+000 |
| 8.450 | 2.51600e+000 | 1.37943e+000 | 2.52489e+000 | 1.30581e+000 | 2.54022e+000 | 1.23539e+000 |
| 8.500 | 2.51772e+000 | 1.38039e+000 | 2.52661e+000 | 1.30673e+000 | 2.54194e+000 | 1.23627e+000 |
| 8.550 | 2.51943e+000 | 1.38135e+000 | 2.52832e+000 | 1.30764e+000 | 2.54364e+000 | 1.23713e+000 |
| 8.600 | 2.52114e+000 | 1.38230e+000 | 2.53001e+000 | 1.30854e+000 | 2.54533e+000 | 1.23800e+000 |
| 8.650 | 2.52282e+000 | 1.38324e+000 | 2.53169e+000 | 1.30944e+000 | 2.54700e+000 | 1.23885e+000 |
| 8.700 | 2.52447e+000 | 1.38417e+000 | 2.53334e+000 | 1.31033e+000 | 2.54865e+000 | 1.23970e+000 |
| 8.750 | 2.52612e+000 | 1.38508e+000 | 2.53499e+000 | 1.31120e+000 | 2.55030e+000 | 1.24053e+000 |
| 8.800 | 2.52774e+000 | 1.38599e+000 | 2.53661e+000 | 1.31207e+000 | 2.55192e+000 | 1.24136e+000 |
| 8.850 | 2.52935e+000 | 1.38689e+000 | 2.53821e+000 | 1.31292e+000 | 2.55352e+000 | 1.24217e+000 |
| 8.900 | 2.53095e+000 | 1.38777e+000 | 2.53980e+000 | 1.31377e+000 | 2.55510e+000 | 1.24298e+000 |
| 8.950 | 2.53252e+000 | 1.38865e+000 | 2.54137e+000 | 1.31460e+000 | 2.55667e+000 | 1.24377e+000 |
| 9.000 | 2.53407e+000 | 1.38951e+000 | 2.54292e+000 | 1.31543e+000 | 2.55821e+000 | 1.24456e+000 |
| 9.050 | 2.53561e+000 | 1.39037e+000 | 2.54445e+000 | 1.31625e+000 | 2.55974e+000 | 1.24534e+000 |
| 9.100 | 2.53713e+000 | 1.39123e+000 | 2.54597e+000 | 1.31706e+000 | 2.56126e+000 | 1.24612e+000 |
| 9.150 | 2.53864e+000 | 1.39206e+000 | 2.54747e+000 | 1.31786e+000 | 2.56277e+000 | 1.24688e+000 |
| 9.200 | 2.54013e+000 | 1.39289e+000 | 2.54896e+000 | 1.31865e+000 | 2.56424e+000 | 1.24763e+000 |
| 9.250 | 2.54160e+000 | 1.39372e+000 | 2.55042e+000 | 1.31944e+000 | 2.56571e+000 | 1.24838e+000 |
| 9.300 | 2.54305e+000 | 1.39453e+000 | 2.55188e+000 | 1.32022e+000 | 2.56716e+000 | 1.24912e+000 |
| 9.350 | 2.54450e+000 | 1.39533e+000 | 2.55332e+000 | 1.32098e+000 | 2.56860e+000 | 1.24985e+000 |
| 9.400 | 2.54593e+000 | 1.39613e+000 | 2.55475e+000 | 1.32174e+000 | 2.57002e+000 | 1.25058e+000 |
| 9.450 | 2.54736e+000 | 1.39692e+000 | 2.55617e+000 | 1.32250e+000 | 2.57144e+000 | 1.25130e+000 |
| 9.500 | 2.54877e+000 | 1.39771e+000 | 2.55758e+000 | 1.32325e+000 | 2.57285e+000 | 1.25201e+000 |
| 9.550 | 2.55017e+000 | 1.39850e+000 | 2.55897e+000 | 1.32400e+000 | 2.57424e+000 | 1.25273e+000 |
| 9.600 | 2.55156e+000 | 1.39927e+000 | 2.56036e+000 | 1.32474e+000 | 2.57563e+000 | 1.25343e+000 |
| 9.650 | 2.55293e+000 | 1.40004e+000 | 2.56173e+000 | 1.32547e+000 | 2.57700e+000 | 1.25413e+000 |
| 9.700 | 2.55430e+000 | 1.40080e+000 | 2.56309e+000 | 1.32620e+000 | 2.57835e+000 | 1.25482e+000 |
| 9.750 | 2.55565e+000 | 1.40155e+000 | 2.56444e+000 | 1.32691e+000 | 2.57970e+000 | 1.25550e+000 |
| 9.800 | 2.55699e+000 | 1.40229e+000 | 2.56577e+000 | 1.32763e+000 | 2.58102e+000 | 1.25618e+000 |
| 9.850 | 2.55830e+000 | 1.40303e+000 | 2.56708e+000 | 1.32833e+000 | 2.58233e+000 | 1.25685e+000 |
| 9.900 | 2.55961e+000 | 1.40376e+000 | 2.56839e+000 | 1.32903e+000 | 2.58364e+000 | 1.25751e+000 |
| 9.950 | 2.56090e+000 | 1.40448e+000 | 2.56968e+000 | 1.32971e+000 | 2.58493e+000 | 1.25817e+000 |
| 10.000 | 2.56219e+000 | 1.40520e+000 | 2.57096e+000 | 1.33039e+000 | 2.58621e+000 | 1.25882e+000 |
